# Supplementary material for: A fast algorithm with minimax optimal guarantees for topic models with an unknown number of topics
Source: arXiv:1805.06837 source file (2019-09-04)
Supplement: Supplementary file 1 [file supp.pdf]

# Supplement to “A fast algorithm with minimax optimal guarantees for topic models with an unknown number of topics”

XIN BING<sup>1,\*</sup> FLORENTINA BUNEA<sup>1,\*\*</sup> and MARTEN WEGKAMP<sup>1,2</sup>

<sup>1</sup>*Department of Statistical Science, Cornell University, Ithaca, New York, USA.*

*E-mail:* <sup>\*</sup>[xb43@cornell.edu](mailto:xb43@cornell.edu); <sup>\*\*</sup>[fb238@cornell.edu](mailto:fb238@cornell.edu)

<sup>2</sup>*Department of Mathematics, Cornell University, Ithaca, New York, USA.*

*E-mail:* [mhw73@cornell.edu](mailto:mhw73@cornell.edu)

From the topic model specifications, the matrices  $\Pi$ ,  $A$  and  $W$  are all scaled as

$$\sum_{j=1}^p \Pi_{ji} = 1, \quad \sum_{j=1}^p A_{jk} = 1, \quad \sum_{k=1}^K W_{ki} = 1 \quad (1)$$

for any  $1 \leq j \leq p$ ,  $1 \leq i \leq n$  and  $1 \leq k \leq K$ . In order to adjust their scales properly, we denote

$$m_j = p \max_{1 \leq i \leq n} \Pi_{ji}, \quad \mu_j = \frac{p}{n} \sum_{i=1}^n \Pi_{ji}, \quad \alpha_j = p \max_{1 \leq k \leq K} A_{jk}, \quad \gamma_k = \frac{K}{n} \sum_{i=1}^n W_{ki}, \quad (2)$$

so that

$$\sum_{k=1}^K \gamma_k = K, \quad \sum_{j=1}^p \mu_j = p. \quad (3)$$

We further denote  $m_{\min} = \min_{1 \leq j \leq p} m_j$  and  $\mu_{\min} = \min_{1 \leq j \leq p} \mu_j$ .

## Appendix A: Proofs of Section 2

**Proof of Proposition 1.** Recall that  $Y_i := N_i X_i \sim \text{Multinomial}_p(N_i; \Pi_i)$  for any  $i \in [n]$ . The joint log-likelihood of  $(Y_1, \dots, Y_n)$  is

$$\begin{aligned} \ell(Y_1, \dots, Y_n) &= \sum_{i=1}^n \log(N_i!) - \sum_{i=1}^n \sum_{j=1}^p \log(Y_{ji}) + \sum_{i=1}^n \sum_{j=1}^p Y_{ji} \log \Pi_{ji} \\ &= \sum_{i=1}^n \log(N_i!) - \sum_{i=1}^n \sum_{j=1}^p \log(Y_{ji}) + \sum_{i=1}^n \sum_{j=1}^p Y_{ji} \log \left( \sum_{k=1}^K A_{jk} W_{ki} \right). \end{aligned}$$

Fix any  $j \in [p]$ ,  $k \in [K]$  and  $i \in [n]$ . It follows that

$$\frac{\partial \ell(Y_1, \dots, Y_n)}{\partial A_{jk}} = \begin{cases} \sum_{i=1}^n Y_{ji} W_{ki} / \left( \sum_{t=1}^K A_{jt} W_{ti} \right), & \text{if } A_{jk} \neq 0, W_{ki} \neq 0 \\ 0, & \text{otherwise} \end{cases}$$

from which we further deduce

$$\begin{aligned} & \frac{\partial^2 \ell(Y_1, \dots, Y_n)}{\partial A_{jk} \partial W_{ki}} \\ &= \begin{cases} \sum_{i=1}^n Y_{ji} \left( \sum_{t=1}^K A_{jt} W_{ti} - A_{jk} W_{ki} \right) / \left( \sum_{t=1}^K A_{jt} W_{ti} \right)^2, & \text{if } A_{jk} \neq 0, W_{ki} \neq 0 \\ 0, & \text{otherwise} \end{cases}. \end{aligned}$$

Since  $\mathbb{E}[Y_{ji}] = N_i \Pi_{ji}$ , taking expectation yields

$$\begin{aligned} & \mathbb{E} \left[ -\frac{\partial^2 \ell(Y_1, \dots, Y_n)}{\partial A_{jk} \partial W_{ki}} \right] \\ &= \begin{cases} \sum_{i=1}^n N_i \left( \sum_{t \neq k} A_{jt} W_{ti} \right) / \left( \sum_{t=1}^K A_{jt} W_{ti} \right), & \text{if } A_{jk} \neq 0, W_{ki} \neq 0 \\ 0, & \text{otherwise} \end{cases}. \end{aligned} \quad (4)$$

Similarly, for this  $j$ ,  $k$  and  $i$  but with any  $k' \neq k$ , we have

$$\begin{aligned} & \frac{\partial^2 \ell(Y_1, \dots, Y_n)}{\partial A_{jk} \partial W_{k'i}} \\ &= \begin{cases} -\sum_{i=1}^n Y_{ji} A_{jk'} W_{ki} / \left( \sum_{t=1}^K A_{jt} W_{ti} \right)^2, & \text{if } A_{jk} \neq 0, A_{jk'} \neq 0, W_{k'i} \neq 0, W_{ki} \neq 0 \\ 0, & \text{otherwise} \end{cases} \end{aligned}$$

and

$$\begin{aligned} & \mathbb{E} \left[ -\frac{\partial^2 \ell(Y_1, \dots, Y_n)}{\partial A_{jk} \partial W_{k'i}} \right] \\ &= \begin{cases} \sum_{i=1}^n N_i A_{jk'} W_{ki} / \sum_{t=1}^K A_{jt} W_{ti}, & \text{if } A_{jk} \neq 0, A_{jk'} \neq 0, W_{k'i} \neq 0, W_{ki} \neq 0 \\ 0, & \text{otherwise} \end{cases}. \end{aligned} \quad (5)$$

From (4) and (5), it is easy to see that condition (7) implies

$$\mathbb{E} \left[ -\frac{\partial^2 \ell(Y_1, \dots, Y_n)}{\partial A_{jk} \partial W_{k'i}} \right] = 0 \quad (6)$$

for any  $j \in [p]$ ,  $k, k' \in [K]$  and  $i \in [n]$ . This proves the sufficiency. To show the necessity, we use contradiction. If (6) holds for any  $j \in [p]$ ,  $k, k' \in [K]$  and  $i \in [n]$ , suppose there exist at least one  $j \in [p]$  and  $i \in [n]$  such that  $\text{supp}(A_{j\cdot}) \cap \text{supp}(W_{\cdot i}) = \{k_1, k_2\}$  and  $k_1 \neq k_2$ . Then, (5) implies

$$\mathbb{E} \left[ -\frac{\partial^2 \ell(Y_1, \dots, Y_n)}{\partial A_{jk_1} \partial W_{k_2 i}} \right] \geq \frac{N_i A_{jk_1} W_{k_2 i}}{A_{jk_1} W_{k_1 i} + A_{jk_2} W_{k_2 i}} \neq 0.$$

This contradicts (7) and concludes the proof.  $\square$

**Proof of Proposition 2.** Since the columns of  $A$  sum up to 1, and Assumption 1 holds, then the matrix  $\tilde{A}$  satisfies:

$$\tilde{A}_{jk} \geq 0, \quad \|\tilde{A}_{j\cdot}\|_1 = 1, \quad \text{for each } j = 1, \dots, p, \text{ and } K = 1, \dots, K. \quad (7)$$

Additionally,  $\tilde{A}$  has the same sparsity pattern as  $A$ , and thus  $\tilde{A}$  satisfies Assumption 1, with the same  $I$  and  $\mathcal{I}$ . We further notice that Assumption 3 is equivalent to

$$|\langle \tilde{W}_i, \tilde{W}_j \rangle| < \|\tilde{W}_i\|^2 \wedge \|\tilde{W}_j\|^2, \quad \text{for all } 1 \leq i < j \leq K,$$

which is further equivalent with  $\nu > 0$ , defined in (23).

To finish the proof we invoke Theorem 1 in [2], slightly adapted to our situation. Specifically, we consider any matrix  $R$  defined in (11) that factorizes as  $R = \tilde{A}\tilde{C}\tilde{A}^T$  where  $\tilde{A}$  satisfies Assumption 1 and  $\tilde{C}$  satisfies (23). Note that the quantities  $M_i$  and  $S_i$  defined in page 9 of [2] are replaced by, respectively,  $T_i$  and  $S_i$  in (12). We proceed to prove (a) and (b) of Proposition 2.

**Proof of (a).** We first show the sufficiency part. Consider any  $i \in [p]$  with  $T_i = T_j$  for all  $j \in S_i$ . Part (a) of Lemma 2, stated after the proof, states that there exists a  $j \in I_a \cap S_i$  for some  $a \in [K]$ . For this  $j \in I_a$ , we have  $T_j = \tilde{C}_{aa}$  from part (b) of Lemma 2. Invoking our premise  $T_j = T_i$  as  $j \in S_i$ , we conclude that  $T_i = \tilde{C}_{aa}$ , that is,  $\max_{k \in p} R_{ik} = \tilde{C}_{aa}$ . By Lemma 1, stated after the proof, the maximum is achieved for any  $i \in I_a$ . However, if  $i \notin I_a$ , we have that  $R_{ik} < \tilde{C}_{aa}$  for all  $k \in [p]$ . Hence  $i \in I_a$  and this concludes the proof of the sufficiency part.

It remains to prove the necessity part. Let  $i \in I_a$  for some  $a \in [K]$  and  $j \in S_i$ . Lemma 2 implies that  $j \in I_a$  and  $T_i = \tilde{C}_{aa}$ . Since  $j \in S_i$ , we have  $R_{ij} = T_i = \tilde{C}_{aa}$ , while  $j \in I_a$  yields  $R_{jk} \leq \tilde{C}_{aa}$  for all  $k \in [p]$ , and  $R_{jk} = \tilde{C}_{aa}$  for  $k \in I_a$ , as a result of Lemma 1. Hence,  $T_j = \max_{k \in [p]} R_{jk} = \tilde{C}_{aa} = T_i$  for any  $j \in S_i$ , which proves our claim.

**Proof of (b).** The proof of (b) follows by the same arguments for proving part (b) of Theorem 1 in [2]. The proof is then complete.  $\square$

The following two lemmas are used in the above proof. They are adapted from Lemmas 1 and 2 of the supplement of [2].

**Lemma 1.** For any  $a \in [K]$  and  $i \in I_a$ , we have

- (a)  $R_{ij} = \tilde{C}_{aa}$  for all  $j \in I_a$ ,
- (b)  $R_{ij} < \tilde{C}_{aa}$  for all  $j \notin I_a$ .

**Proof.** The proof follows the same argument for proving Lemma 1 in [2].  $\square$

**Lemma 2.** Let  $T_i$  and  $S_i$  be defined in (12). We have

- (a)  $S_i \cap I \neq \emptyset$ , for any  $i \in [p]$ ,
- (b)  $S_i \cup \{i\} = I_a$  and  $T_i = \tilde{C}_{aa}$ , for any  $i \in I_a$  and  $a \in [K]$ .

**Proof.** Lemma 1 implies that, for any  $i \in I_a$ ,  $T_i = \tilde{C}_{aa}$  and  $S_i = I_a$ , which proves part (b). Part (a) follows from the result of part (b) and the same arguments of the proof of Lemma 2 in [2] by replacing  $M_i$  by  $T_i$ ,  $|\Sigma_{ij}|$  by  $R_{ij}$ ,  $A$  by  $\tilde{A}$  and  $C$  by  $\tilde{C}$ .  $\square$

## Appendix B: Error bounds of stochastic errors

We use this section to present tight bounds on the error terms which are critical to our later estimation rate. We recall that  $\varepsilon_{ji} := X_{ji} - \Pi_{ji}$ , for  $1 \leq i \leq n$  and  $1 \leq j \leq p$  and assume  $N_1 = \dots = N_n = N$  for ease of presentation since similar results for different  $N$  can be derived by using the same arguments. The following results, Lemmata 5 - 7 control several terms related with  $\varepsilon_{ji}$  under the multinomial assumption (2). We start by stating the well-known Bernstein inequality and Hoeffding inequality for bounded random variables which are used in the sequel.

**Lemma 3** (Bernstein's inequality for bounded random variable). *For independent random variables  $Y_1, \dots, Y_n$  with bounded ranges  $[-B, B]$  and zero means,*

$$\mathbb{P} \left\{ \frac{1}{n} \left| \sum_{i=1}^n Y_i \right| > x \right\} \leq 2 \exp \left( -\frac{n^2 x^2 / 2}{v + n B x / 3} \right), \quad \text{for any } x \geq 0,$$

where  $v \geq \text{var}(Y_1 + \dots + Y_n)$ .

**Lemma 4** (Hoeffding's inequality). *Let  $Y_1, \dots, Y_n$  be independent random variables with  $\mathbb{E}[Y_i] = 0$  and bounded by  $[a_i, b_i]$ : For any  $t \geq 0$ , we have*

$$\mathbb{P} \left\{ \left| \sum_{i=1}^n Y_i \right| > t \right\} \leq 2 \exp \left( -\frac{2t^2}{\sum_{i=1}^n (b_i - a_i)^2} \right).$$

**Lemma 5.** *Assume  $\mu_{\min}/p \geq 2 \log M / (3N)$ . With probability  $1 - 2M^{-1}$ ,*

$$\frac{1}{n} \left| \sum_{i=1}^n \varepsilon_{ji} \right| \leq 2 \sqrt{\frac{\mu_j \log M}{npN}} \left( 1 + \sqrt{6} n^{-\frac{1}{2}} \right), \quad \text{uniformly in } 1 \leq j \leq p.$$

**Proof.** Fix  $1 \leq j \leq p$ . From model (3), we know  $NX_{ji} \sim \text{Binomial}(N; \Pi_{ji})$ . We express the binomial random variable as a sum of i.i.d. Bernoulli random variables:

$$\varepsilon_{ji} = X_{ji} - \Pi_{ji} = \frac{1}{N} \sum_{k=1}^N (B_{ik}^j - \Pi_{ji}) := \frac{1}{N} \sum_{\ell=1}^N Z_{ik}^j$$

with  $B_{i\ell}^j \sim \text{Bernoulli}(\Pi_{ji})$ , such that  $N \sum_{i=1}^n \varepsilon_{ji} = \sum_{i=1}^n \sum_{\ell=1}^N Z_{i\ell}^j$ . Note that  $|Z_{ik}^j| \leq 1$ ,  $\mathbb{E}[Z_{ik}^j] = 0$  and  $\mathbb{E}[(Z_{ik}^j)^2] = \Pi_{ji}(1 - \Pi_{ji}) \leq \Pi_{ji}$ , for all  $i \in [n]$  and  $k \in [N]$ . An application

of Bernstein's inequality, see Lemma 3, to  $Z_{i\ell}^j$  with  $v = N \sum_{i=1}^n \Pi_{ji} = Nn\mu_j/p$  and  $B = 1$  gives

$$\mathbb{P} \left\{ \frac{1}{n} \left| \sum_{i=1}^n \varepsilon_{ji} \right| > t \right\} \leq 2 \exp \left( - \frac{n^2 N^2 t^2 / 2}{N \sum_{i=1}^n \Pi_{ji} + nNt/3} \right), \quad \text{for any } t > 0.$$

This implies, for all  $t > 0$

$$\mathbb{P} \left\{ \frac{1}{n} \left| \sum_{i=1}^n \varepsilon_{ji} \right| > \sqrt{\frac{\mu_j t}{npN}} + \frac{t}{nN} \right\} \leq 2e^{-t/2}.$$

Choosing  $t = 4 \log M$  and recalling that  $M = n \vee N \vee p \geq p$ , we find by the union bound

$$\sum_{j=1}^p \mathbb{P} \left\{ \frac{1}{n} \left| \sum_{i=1}^n \varepsilon_{ji} \right| > 2\sqrt{\frac{\mu_j \log M}{npN}} + \frac{4 \log M}{nN} \right\} \leq 2pM^{-2} \leq 2M^{-1}. \quad (8)$$

Using  $\mu_{\min}/p \geq 2 \log M/(3N)$  concludes the proof.  $\square$

**Remark 1.** By inspection of the proof of Lemma 5, if instead of the bound  $\mathbb{E}[(Z_{ik}^j)^2] \leq \Pi_{ji}$ , we had used the overall bound  $\mathbb{E}[(Z_{ik}^j)^2] \leq 1$ , and application of Bernstein's inequality would yield,

$$\frac{1}{n} \left| \sum_{i=1}^n \varepsilon_{ji} \right| \leq c \sqrt{\frac{\log M}{nN}}, \quad \text{uniformly in } 1 \leq j \leq p.$$

Summing over  $1 \leq j \leq p$  in the above display would further give

$$\frac{1}{n} \sum_{j=1}^p \left| \sum_{i=1}^n \varepsilon_{ji} \right| \leq c \cdot p \sqrt{\frac{\log M}{nN}},$$

and the right hand side would be slower by an important  $\sqrt{p}$  factor than what we would obtain by summing the bound in Lemma 5 over  $1 \leq j \leq p$ , since

$$2 \sum_{j=1}^p \sqrt{\frac{\mu_j \log M}{npN}} \leq 2 \sqrt{\frac{\log M}{nN}} \sqrt{\sum_{j=1}^p \mu_j} = 2 \sqrt{\frac{p \log M}{nN}}.$$

In this last display, we used the Cauchy-Schwarz inequality in the first inequality, and the constraint (3) in the last equality. The bound of Lemma 5 is an important intermediate step for deriving the final bounds of Theorem 7, and the simple calculations presented above that the constraints of unit column sums induced by model (3) permit a more refined control of the stochastic errors than those previously considered. A larger impact of this refinement on the final rate of convergence is illustrated in Remark 2, following the proof of Lemma 7, in which we control sums of quadratic, dependent terms  $\varepsilon_{ji}\varepsilon_{\ell i}$ .

**Lemma 6.** *With probability  $1 - 2M^{-1}$ ,*

$$\frac{1}{n} \left| \sum_{i=1}^n \Pi_{\ell i} \varepsilon_{ji} \right| \leq \sqrt{\frac{6m_\ell \Theta_{j\ell} \log M}{npN}} + \frac{2m_\ell \log M}{npN}, \quad \text{uniformly in } 1 \leq j, \ell \leq p.$$

**Proof.** Similar as in the proof of Lemma 5, we write

$$\Pi_{\ell i} \varepsilon_{ji} = \frac{1}{N} \sum_{k=1}^N \Pi_{\ell i} Z_{ik}^j$$

such that  $|\Pi_{\ell i} Z_{ik}^j| \leq \Pi_{\ell i} \leq m_\ell/p$  by (2),  $\mathbb{E}[\Pi_{\ell i} Z_{ik}^j] = 0$  and  $\mathbb{E}[\Pi_{\ell i}^2 Z_{ik}^2] = \Pi_{\ell i}^2 \Pi_{ji}(1 - \Pi_{ji}) \leq m_\ell \Pi_{\ell i} \Pi_{ji}/p$ , for all  $i \in [n]$  and  $k \in [N]$ . Fix  $1 \leq j, \ell \leq p$  and recall that  $\Theta_{j\ell} = n^{-1} \sum_{i=1}^n \Pi_{ji} \Pi_{\ell i}$ . Applying Bernstein's inequality to  $\Pi_{\ell i} Z_{ik}^j$  with  $v = nNm_\ell \Theta_{j\ell}/p$  and  $B = m_\ell/p$  gives

$$\mathbb{P} \left\{ \frac{1}{n} \left| \sum_{i=1}^n \Pi_{\ell i} \varepsilon_{ji} \right| \geq t \right\} \leq 2 \exp \left( - \frac{n^2 N^2 t^2 / 2}{nNm_\ell \Theta_{j\ell}/p + nNm_\ell t/(3p)} \right)$$

which further implies

$$\mathbb{P} \left\{ \frac{1}{n} \left| \sum_{i=1}^n \Pi_{\ell i} \varepsilon_{ji} \right| > \sqrt{\frac{m_\ell \Theta_{j\ell} t}{npN}} + \frac{m_\ell t}{3npN} \right\} \leq 2e^{-t/2}.$$

Taking the union bound over  $1 \leq j, \ell \leq p$ , and choosing  $t = 6 \log M$ , concludes the proof.  $\square$

**Lemma 7.** *If  $\mu_{\min}/p \geq 2 \log M/(3N)$ , then with probability  $1 - 4M^{-1}$ ,*

$$\frac{1}{n} \left| \sum_{i=1}^n (\varepsilon_{ji} \varepsilon_{\ell i} - \mathbb{E}[\varepsilon_{ji} \varepsilon_{\ell i}]) \right| \leq 12\sqrt{6} \sqrt{\Theta_{j\ell} + \frac{(\mu_j + \mu_\ell) \log M}{pN}} \sqrt{\frac{(\log M)^3}{nN^2}} + 4M^{-3},$$

*holds, uniformly in  $1 \leq j, \ell \leq p$ .*

**Proof.** For any  $1 \leq j \leq p$ , recall that  $\varepsilon_{ji} = X_{ji} - \Pi_{ji}$  and

$$\varepsilon_{ji} = \frac{1}{N} \sum_{k=1}^N Z_{ik}^j$$

where  $Z_{ik}^j := B_{ik}^j - \Pi_{ji}$  and  $B_{ik}^j \sim \text{Bernoulli}(\Pi_{ji})$ . By using the arguments of Lemma 5, application of Bernstein's inequality to  $Z_{ik}^j$  with  $v = N\Pi_{ji}$  and  $B = 1$  gives

$$\mathbb{P} \{ |\varepsilon_{ji}| > t \} \leq 2 \exp \left( - \frac{Nt^2/2}{\Pi_{ji} + t/3} \right), \quad \text{for any } t > 0,$$

which yields

$$|\varepsilon_{ji}| \leq \sqrt{\frac{6\Pi_{ji} \log M}{N}} + \frac{2 \log M}{N} := T_{ji}$$

with probability greater than  $1 - 2M^{-3}$ . We define  $Y_{ji} = \varepsilon_{ji} \mathbb{1}_{\mathcal{S}_{ji}}$  with  $\mathcal{S}_{ji} := \{|\varepsilon_{ji}| \leq T_{ji}\}$  for each  $1 \leq j \leq p$  and  $1 \leq i \leq n$ , and  $\mathcal{S} := \cap_{j=1}^p \cap_{i=1}^n \mathcal{S}_{ji}$ . It follows that  $\mathbb{P}(\mathcal{S}_{ji}) \geq 1 - 2M^{-3}$  for all  $1 \leq i \leq n$  and  $1 \leq j \leq p$ , so that  $\mathbb{P}(\mathcal{S}) \geq 1 - 2M^{-1}$  as  $M := n \vee p \vee N$ . On the event  $\mathcal{S}$ , we have

$$\frac{1}{n} \left| \sum_{i=1}^n (\varepsilon_{ji} \varepsilon_{\ell i} - \mathbb{E}[\varepsilon_{ji} \varepsilon_{\ell i}]) \right| \leq \underbrace{\frac{1}{n} \left| \sum_{i=1}^n (Y_{ji} Y_{\ell i} - \mathbb{E}[Y_{ji} Y_{\ell i}]) \right|}_{T_1} + \underbrace{\frac{1}{n} \left| \sum_{i=1}^n (\mathbb{E}[\varepsilon_{ji} \varepsilon_{\ell i}] - \mathbb{E}[Y_{ji} Y_{\ell i}]) \right|}_{T_2}$$

We first study  $T_2$ . By writing

$$\mathbb{E}[\varepsilon_{ji} \varepsilon_{\ell i}] = \mathbb{E}[Y_{ji} Y_{\ell i}] + \mathbb{E}[Y_{ji} \varepsilon_{\ell i} \mathbb{1}_{\mathcal{S}_{\ell i}^c}] + \mathbb{E}[\varepsilon_{ji} \mathbb{1}_{\mathcal{S}_{ji}^c} \varepsilon_{\ell i}],$$

we have

$$\begin{aligned} T_2 &= \frac{1}{n} \left| \sum_{i=1}^n (\mathbb{E}[\varepsilon_{ji} \varepsilon_{\ell i}] - \mathbb{E}[Y_{ji} Y_{\ell i}]) \right| \leq \frac{1}{n} \left| \sum_{i=1}^n \left( \mathbb{E}[Y_{ji} \varepsilon_{\ell i} \mathbb{1}_{\mathcal{S}_{\ell i}^c}] + \mathbb{E}[\varepsilon_{ji} \mathbb{1}_{\mathcal{S}_{ji}^c} \varepsilon_{\ell i}] \right) \right| \\ &\leq \frac{1}{n} \left| \sum_{i=1}^n (\mathbb{P}(\mathcal{S}_{ji}^c) + \mathbb{P}(\mathcal{S}_{\ell i}^c)) \right| \\ &\leq 4M^{-3} \end{aligned} \tag{9}$$

by using  $|Y_{ji}| \leq |\varepsilon_{ji}| \leq 1$  in the second inequality.

Next we bound  $T_1$ . Since  $|Y_{ji}| \leq T_{ji}$ , we know  $-2T_{ji}T_{\ell i} \leq Y_{ji}Y_{\ell i} - \mathbb{E}[Y_{ji}Y_{\ell i}] \leq 2T_{ji}T_{\ell i}$  for all  $1 \leq i \leq n$ . Applying the Hoeffding inequality Lemma 4 with  $a_i = -2T_{ji}T_{\ell i}$  and  $b_i = 2T_{ji}T_{\ell i}$  gives

$$\mathbb{P} \left\{ \left| \sum_{i=1}^n (Y_{ji} Y_{\ell i} - \mathbb{E}[Y_{ji} Y_{\ell i}]) \right| \geq t \right\} \leq 2 \exp \left( -\frac{t^2}{8 \sum_{i=1}^n T_{ji}^2 T_{\ell i}^2} \right).$$

Taking  $t = \sqrt{24 \sum_{i=1}^n T_{ji}^2 T_{\ell i}^2 \log M}$  yields

$$T_1 = \frac{1}{n} \left| \sum_{i=1}^n (Y_{ji} Y_{\ell i} - \mathbb{E}[Y_{ji} Y_{\ell i}]) \right| \leq 2\sqrt{6} \left( \frac{1}{n} \sum_{i=1}^n T_{ji}^2 T_{\ell i}^2 \cdot \frac{\log M}{n} \right)^{1/2} \tag{10}$$

with probability greater than  $1 - 2M^{-3}$ . Finally, note that

$$\begin{aligned} \frac{1}{n} \sum_{i=1}^n T_{ji}^2 T_{\ell i}^2 &= \frac{1}{n} \sum_{i=1}^n \left( \Pi_{ji} \Pi_{\ell i} \frac{36(\log M)^2}{N^2} + \left( \frac{2 \log M}{N} \right)^4 + (\Pi_{ji} + \Pi_{\ell i}) \frac{24(\log M)^3}{N^3} \right) \\ &= 36\Theta_{j\ell} \left( \frac{\log M}{N} \right)^2 + 16 \left( \frac{\log M}{N} \right)^4 + 24(\mu_j + \mu_\ell) \frac{(\log M)^3}{pN^3} \end{aligned} \tag{11}$$

by using (2) and  $\Theta_{j\ell} = n^{-1}\Pi\Pi^T$  in the second equality. Finally, combining (9) - (11) and using  $\mu_{\min}/p \geq 2\log M/(3N)$  conclude the proof.  $\square$

**Remark 2.** We illustrate the improvement of our result over a simple application of Hanson-Wright inequality. Write

$$4\varepsilon_{ji}\varepsilon_{\ell i} = (\varepsilon_{ji} + \varepsilon_{\ell i})^2 - (\varepsilon_{ji} - \varepsilon_{\ell i})^2$$

for each  $i \in [n]$ . Since  $\varepsilon_{ji} = N^{-1} \sum_{k=1}^N Z_{ik}^j$  and  $\|\varepsilon_{ji} \pm \varepsilon_{\ell i}\|_{\phi_2} \leq 2/\sqrt{N}$ , a direct application of the Hanson-Wright inequality to the two terms in the right hand side will give

$$\frac{1}{n} \left| \sum_{i=1}^n (\varepsilon_{ji}\varepsilon_{\ell i} - \mathbb{E}[\varepsilon_{ji}\varepsilon_{\ell i}]) \right| \leq c \sqrt{\frac{\log M}{nN}}$$

with high probability. Summing over  $1 \leq j \leq p$  and  $1 \leq \ell \leq p$  further yields

$$\sum_{j,\ell=1}^p \frac{1}{n} \left| \sum_{i=1}^n (\varepsilon_{ji}\varepsilon_{\ell i} - \mathbb{E}[\varepsilon_{ji}\varepsilon_{\ell i}]) \right| \leq c \cdot p^2 \sqrt{\frac{\log M}{nN}}. \quad (12)$$

By contrast, summing the first term in Lemma 7 yields

$$\begin{aligned} \sum_{j,\ell=1}^p \frac{1}{n} \left| \sum_{i=1}^n (\varepsilon_{ji}\varepsilon_{\ell i} - \mathbb{E}[\varepsilon_{ji}\varepsilon_{\ell i}]) \right| &\leq c \cdot \sqrt{\frac{p^2(\log M)^3}{nN^2}} \sqrt{\sum_{1 \leq j,\ell \leq p} \Theta_{j\ell}} + c \cdot \sqrt{\frac{p^3(\log M)^4}{nN^3}} \\ &= c \cdot \sqrt{\frac{p^2(\log M)^3}{nN^2}} + c \cdot \sqrt{\frac{p^3(\log M)^4}{nN^3}} \end{aligned}$$

by using Cauchy-Schwarz in the first inequality and (1) in the last equality which is  $(p\sqrt{N}) \wedge (N\sqrt{p})$  faster than the result in (12) after ignoring the logarithmic term.

## Appendix C: Proofs of Section 4

Throughout this section, we define the event  $\mathcal{E} := \mathcal{E}_1 \cap \mathcal{E}_2 \cap \mathcal{E}_3$  by

$$\begin{aligned} \mathcal{E}_1 &= \bigcap_{j=1}^p \left\{ \frac{1}{n} \left| \sum_{i=1}^n \varepsilon_{ji} \right| \leq 2(1 + \sqrt{6/n}) \sqrt{\frac{\mu_j \log M}{npN}} \right\}, \\ \mathcal{E}_2 &= \bigcap_{j,\ell=1}^p \left\{ \frac{1}{n} \left| \sum_{i=1}^n \Pi_{\ell i} \varepsilon_{ji} \right| \leq \sqrt{\frac{6m_\ell \Theta_{j\ell} \log M}{npN}} + \frac{2m_\ell \log M}{npN} \right\}, \\ \mathcal{E}_3 &= \bigcap_{j,\ell=1}^p \left\{ \frac{1}{n} \left| \sum_{i=1}^n (\varepsilon_{ji}\varepsilon_{\ell i} - \mathbb{E}[\varepsilon_{ji}\varepsilon_{\ell i}]) \right| \leq 12\sqrt{6} \sqrt{\Theta_{j\ell} + \frac{(\mu_j + \mu_\ell) \log M}{pN}} \sqrt{\frac{(\log M)^3}{nN^2}} + 4M^{-3} \right\} \end{aligned}$$

Recall (2) and (3), if

$$\min_{1 \leq j \leq p} \frac{1}{n} \sum_{i=1}^n \Pi_{ji} \geq \frac{2 \log M}{3N}$$

holds, we have

$$\frac{1}{p} \geq \frac{\mu_{\min}}{p} = \min_{1 \leq j \leq p} \frac{1}{n} \sum_{i=1}^n \Pi_{ji} \geq \frac{2 \log M}{3N}, \quad (13)$$

Therefore, invoking Lemmas 5 – 7 yields  $\mathbb{P}(\mathcal{E}) \geq 1 - 8M^{-1}$ .

### C.1. Preliminaries

From model specifications (1) and (2), we first give some useful expressions which are repeatedly invoked later.

(a) For any  $j \in [p]$ , by using (2),

$$\mu_j = \frac{p}{n} \sum_{i=1}^n \Pi_{ji} = \frac{p}{n} \sum_{i=1}^n \sum_{k=1}^K A_{jk} W_{ki} = \frac{p}{K} \sum_{k=1}^K A_{jk} \gamma_k \Rightarrow \frac{p}{K} \sum_{k=1}^K A_{jk} \cdot \underline{\gamma} \leq \mu_j \leq \alpha_j. \quad (14)$$

In particular, for any  $j \in I_k$  with any  $k \in [K]$ ,

$$\mu_j = \frac{p}{n} \sum_{i=1}^n \sum_{k=1}^K A_{jk} W_{ki} = \frac{p}{K} A_{jk} \gamma_k \stackrel{(2)}{=} \frac{\alpha_j \gamma_k}{K}. \quad (15)$$

(b) For any  $j \in [p]$ ,

$$m_j \stackrel{(2)}{=} p \max_{1 \leq i \leq n} \Pi_{ji} = p \max_{1 \leq i \leq n} \sum_{k=1}^K A_{jk} W_{ki} \leq p \max_{1 \leq k \leq K} A_{jk} \stackrel{(2)}{=} \alpha_j \Rightarrow \mu_j \leq m_j \leq \alpha_j, \quad (16)$$

by using  $0 \leq W_{ki} \leq 1$  and  $\sum_k W_{ki} = 1$  for any  $k \in [K]$  and  $i \in [n]$ .

### C.2. Control of $\hat{\Theta} - \Theta$ and $\hat{R} - R$

**Proposition 8.** *Under model (3), assume (26). Let  $\hat{\Theta}$  and  $\hat{R}$  be defined in (20) and (21), respectively. Then  $\hat{\Theta}$  is an unbiased estimator of  $\Theta$ . Moreover, with probability greater than  $1 - 8M^{-1}$ ,*

$$|\hat{\Theta}_{j\ell} - \Theta_{j\ell}| \leq \eta_{j\ell}, \quad |\hat{R}_{j\ell} - R_{j\ell}| \leq \delta_{j\ell}$$

for all  $1 \leq j, \ell \leq p$ , where

$$\begin{aligned} \eta_{j\ell} := & 3\sqrt{6} \left( \sqrt{\frac{m_j}{p}} + \sqrt{\frac{m_\ell}{p}} \right) \sqrt{\frac{\Theta_{j\ell} \log M}{nN}} + \frac{2(m_j + m_\ell) \log M}{p} \frac{1}{nN} \\ & + 31(1 + \kappa_1) \sqrt{\frac{\mu_j + \mu_\ell}{p} \frac{(\log M)^4}{nN^3}} + \kappa_2 \end{aligned} \quad (17)$$

and

$$\delta_{j\ell} := (1 + \kappa_1 \kappa_3) \frac{p^2}{\mu_j \mu_\ell} \eta_{j\ell} + \kappa_3 \frac{p^2 \Theta_{j\ell}}{\mu_j \mu_\ell} \left( \sqrt{\frac{p}{\mu_j}} + \sqrt{\frac{p}{\mu_\ell}} \right) \sqrt{\frac{\log M}{nN}}, \quad (18)$$

with  $\kappa_1 = \sqrt{6/n}$ ,  $\kappa_2 = 4/M^3$  and

$$\kappa_3 = \frac{2(1 + \kappa_1)}{(1 - \kappa_1 - \kappa_1^2)^2}.$$

**Remark 3.** For ease of presentation, we assumed that the document lengths are equal, that is,  $N_i = N$  for all  $i \in [n]$ . Inspection of the proofs of Lemmas 5 - 7 and Proposition 8, we may allow for unequal document lengths  $N_i$  by adjusting the quantities  $\eta_{j\ell}$  and  $\delta_{j\ell}$  with

$$\begin{aligned} \eta_{j\ell} := & 3\sqrt{6} (\sqrt{m_j} + \sqrt{m_\ell}) \sqrt{\frac{\log M}{np}} \left( \frac{1}{n} \sum_{i=1}^n \frac{\Pi_{ji} \Pi_{\ell i}}{N_i} \right)^{1/2} + \frac{2(m_j + m_\ell) \log M}{np} \left( \frac{1}{n} \sum_{i=1}^n \frac{1}{N_i} \right) \\ & + 31(1 + \kappa_1) \sqrt{\frac{(\log M)^4}{n}} \left( \frac{1}{n} \sum_{i=1}^n \frac{\Pi_{ji} + \Pi_{\ell i}}{N_i^3} \right)^{1/2} + \kappa_2 \end{aligned} \quad (19)$$

$$\delta_{j\ell} := (1 + \kappa_1 \kappa_3) \frac{p^2 \eta_{j\ell}}{\mu_j \mu_\ell} + \kappa_3 \frac{p^3 \Theta_{j\ell}}{\mu_j \mu_\ell} \sqrt{\frac{\log M}{n}} \left[ \left( \frac{1}{n} \sum_{i=1}^n \frac{\Pi_{ji}}{\mu_j^2 N_i} \right)^{1/2} + \left( \frac{1}{n} \sum_{i=1}^n \frac{\Pi_{\ell i}}{\mu_\ell^2 N_i} \right)^{1/2} \right]. \quad (20)$$

The quantities  $m_j$  and  $\mu_j$  appearing in the above rates are related with  $\Pi$  and can be directly estimated from  $X$ . Let

$$\frac{\hat{m}_j}{p} = \max_{1 \leq i \leq n} X_{ji}, \quad \frac{\hat{\mu}_j}{p} = \frac{1}{n} \sum_{i=1}^n X_{ji}. \quad (21)$$

The following corollary gives the data dependent bounds of  $\hat{\Theta} - \Theta$  and  $\hat{R} - R$ .

**Corollary 9.** Under the same conditions as Proposition 8, with probability greater than  $1 - 8M^{-1}$ , we have

$$|\hat{\Theta}_{j\ell} - \Theta_{j\ell}| \leq \hat{\eta}_{j\ell}, \quad |\hat{R}_{j\ell} - R_{j\ell}| \leq \hat{\delta}_{j\ell}, \quad \text{for all } 1 \leq j, \ell \leq p.$$

The quantities  $\hat{\eta}_{j\ell}$  have the same form as (19) and (20) except for replacing  $\Theta_{j\ell}$ ,  $m_j/p$  and  $\mu_j/p$  by  $\hat{\Theta}_{j\ell} + \kappa_5$ ,  $\hat{m}_j/p + \kappa_4$  and  $\hat{\mu}_j/p + \kappa_5$ , respectively, with  $\kappa_4 = O(\sqrt{\log M/N})$  and  $\kappa_5 = O(\sqrt{\log M/(nN)})$ . Similarly,  $\hat{\delta}_{j\ell}$  can be estimated in the same way by replacing  $\eta_{j\ell}$ ,  $(\mu_j/p)^{-1}$  and  $\Theta_{j\ell}$  by  $\hat{\eta}_{j\ell}$ ,  $(\hat{\mu}_j/p - \kappa_5)^{-1}$  and  $\hat{\Theta}_{j\ell} + \kappa_5$ , respectively.

**Proof of Proposition 8.** Throughout the proof, we work on the event  $\mathcal{E}$ . Write  $X = (X_1, \dots, X_n) \in \mathbb{R}^{p \times n}$  and similarly, for  $\varepsilon = (\varepsilon_1, \dots, \varepsilon_n)$  and  $W = (W_1, \dots, W_n)$ . We first show that  $\mathbb{E}[\hat{\Theta}] = \Theta$ . Recall that  $X_i = AW_i + \varepsilon_i$  satisfying

$$\mathbb{E}X_i = AW_i, \quad \text{Cov}(X_i) = \frac{1}{N_i} \text{diag}(AW_i) - \frac{1}{N_i} AW_i W_i^T A^T.$$

This gives

$$\mathbb{E}[\hat{\Theta}] = \frac{1}{n} \sum_{i=1}^n \left[ \frac{N_i}{N_i - 1} \mathbb{E}[X_i X_i^T] - \frac{1}{N_i - 1} \text{diag}(\mathbb{E}X_i) \right] = \frac{1}{n} \sum_{i=1}^n AW_i W_i^T A^T = \Theta.$$

Next we bound the entry-wise error rate of  $\hat{\Theta} - \Theta$ . Observe that

$$\begin{aligned} \hat{\Theta} &= \frac{1}{n} \sum_{i=1}^n \left[ \frac{N_i}{N_i - 1} (AW_i + \varepsilon_i)(AW_i + \varepsilon_i)^T - \frac{1}{N_i - 1} \text{diag}(AW_i + \varepsilon_i) \right] \\ &= \frac{1}{n} \sum_{i=1}^n \left[ \frac{N_i}{N_i - 1} (AW_i W_i^T A^T + AW_i \varepsilon_i^T + \varepsilon_i (AW_i)^T + \varepsilon_i \varepsilon_i^T) - \frac{1}{N_i - 1} \text{diag}(AW_i + \varepsilon_i) \right] \\ &= \frac{1}{n} \sum_{i=1}^n \left[ AW_i W_i^T A^T + \frac{N_i}{N_i - 1} (AW_i \varepsilon_i^T + \varepsilon_i (AW_i)^T) - \frac{\text{diag}(\varepsilon_i)}{N_i - 1} \right. \\ &\quad \left. + \frac{N_i}{N_i - 1} (\varepsilon_i \varepsilon_i^T - \mathbb{E}[\varepsilon_i \varepsilon_i^T]) \right]. \end{aligned}$$

The third equality comes from the fact that

$$\mathbb{E}[\varepsilon_i \varepsilon_i^T] = \frac{1}{N_i} \text{diag}(AW_i) - \frac{1}{N_i} AW_i W_i^T A^T.$$

Recall that  $\Theta = n^{-1} \sum_{i=1}^n AW_i W_i^T A^T$ . We have

$$\begin{aligned} |\hat{\Theta}_{j\ell} - \Theta_{j\ell}| &\leq \underbrace{\left| \frac{1}{n} \sum_{i=1}^n (AW_i \varepsilon_i^T + \varepsilon_i (AW_i)^T)_{j\ell} \right|}_{T_1} + \underbrace{\left| \frac{1}{n} \sum_{i=1}^n \frac{1}{N_i} (\text{diag}(\varepsilon_i))_{j\ell} \right|}_{T_2} \\ &\quad + \underbrace{\left| \frac{1}{n} \sum_{i=1}^n (\varepsilon_{ji} \varepsilon_{\ell i} - \mathbb{E}[\varepsilon_{ji} \varepsilon_{\ell i}]) \right|}_{T_3}. \end{aligned} \tag{22}$$

It remains to bound  $T_1, T_2$  and  $T_3$ . Fix  $1 \leq j, \ell \leq p$ . To bound  $T_1$ , we have

$$T_1 \leq \frac{1}{n} \left| \sum_{i=1}^n \Pi_{ji} \varepsilon_{\ell i} \right| + \frac{1}{n} \left| \sum_{i=1}^n \Pi_{\ell i} \varepsilon_{ji} \right| \stackrel{\varepsilon}{\leq} (\sqrt{m_j} + \sqrt{m_\ell}) \sqrt{\frac{6\Theta_{j\ell} \log M}{npN}} + \frac{2(m_j + m_\ell) \log M}{npN}. \quad (23)$$

For  $T_2$ , we have

$$T_2 = \frac{1}{nN} \left| \sum_{i=1}^n \varepsilon_{ji} \right| \stackrel{\varepsilon}{\leq} 2(1 + \kappa_1) \sqrt{\frac{\mu_j \log M}{npN^3}}, \quad (24)$$

if  $j = \ell$ . Note that  $(T_2)_{j\ell} = 0$  if  $j \neq \ell$ . Finally, to bound  $T_3$ , we obtain

$$\begin{aligned} T_3 &\leq \frac{1}{n} \left| \sum_{i=1}^n (\varepsilon_{ji} \varepsilon_{\ell i} - \mathbb{E}[\varepsilon_{ji} \varepsilon_{\ell i}]) \right| \\ &\stackrel{\varepsilon}{\leq} 12\sqrt{6} \sqrt{\Theta_{j\ell} + \frac{(\mu_j + \mu_\ell) \log M}{pN}} \sqrt{\frac{(\log M)^3}{nN^2}} + \kappa_2 \\ &\leq 12\sqrt{\frac{6\Theta_{j\ell}(\log M)^3}{nN^2}} + 12\sqrt{\frac{6(\mu_j + \mu_\ell)(\log M)^4}{npN^3}} + \kappa_2. \end{aligned} \quad (25)$$

Since (26) implies

$$\frac{m_{\min}}{p} = \min_{1 \leq j \leq p} \max_{1 \leq i \leq n} \Pi_{ji} \geq \frac{(3 \log M)^2}{N} \quad (26)$$

by recalling (2), we have

$$12\sqrt{\frac{6\Theta_{j\ell}(\log M)^3}{nN^2}} + (\sqrt{m_j} + \sqrt{m_\ell}) \sqrt{\frac{6\Theta_{j\ell} \log M}{npN}} \leq 3\sqrt{6}(\sqrt{m_j} + \sqrt{m_\ell}) \sqrt{\frac{\Theta_{j\ell} \log M}{npN}}.$$

In addition,

$$2(1 + \kappa_1) \sqrt{\frac{\mu_j \log M}{npN^3}} \mathbb{1}_{\{j=\ell\}} + 12\sqrt{\frac{6(\mu_j + \mu_\ell)(\log M)^4}{npN^3}} \leq 31(1 + \kappa_1) \sqrt{\frac{(\mu_j + \mu_\ell)(\log M)^4}{npN^3}}.$$

Combining (23) - (25) concludes the desired rate of  $\hat{\Theta} - \Theta$ .

To prove the rate of  $\hat{R} - R$ , recall that  $R = (nD_\Pi^{-1})\Theta(nD_\Pi^{-1})$ . Fix  $1 \leq j, \ell \leq p$ . By using the diagonal structure of  $D_X$  and  $D_\Pi$ , it follows

$$\begin{aligned} &\left[ (nD_X^{-1}) \hat{\Theta} (nD_X^{-1}) - R \right]_{j\ell} \\ &= \underbrace{n^2 (D_X^{-1} - D_\Pi^{-1})_{jj} \hat{\Theta}_{j\ell} (D_X^{-1})_{\ell\ell}}_{T_4} + \underbrace{n^2 (D_\Pi^{-1})_{jj} \hat{\Theta}_{j\ell} (D_X^{-1} - D_\Pi^{-1})_{\ell\ell}}_{T_5} \\ &\quad + \underbrace{n^2 (D_\Pi^{-1})_{jj} (\hat{\Theta} - \Theta)_{j\ell} (D_\Pi^{-1})_{\ell\ell}}_{T_6}. \end{aligned}$$

We first quantify the term  $n(D_X^{-1} - D_\Pi^{-1})$ . From their definitions,

$$\begin{aligned}
n \left| (D_X^{-1} - D_\Pi^{-1})_{jj} \right| &= n \left| \frac{1}{\sum_{i=1}^n \Pi_{ji} + \sum_{i=1}^n \varepsilon_{ji}} - \frac{1}{\sum_{i=1}^n \Pi_{ji}} \right| \\
&\stackrel{(2)}{\leq} \frac{1}{n} \left| \sum_{i=1}^n \varepsilon_{ji} \right| \left/ \left( \frac{\mu_j}{p} \left| \frac{\mu_j}{p} + \frac{1}{n} \sum_{i=1}^n \varepsilon_{ji} \right| \right) \right. \\
&\stackrel{\varepsilon}{\leq} \frac{2(1 + \kappa_1)}{1 - \kappa_1(1 + \kappa_1)} \cdot \frac{p}{\mu_j} \sqrt{\frac{p \log M}{\mu_j n N}}, \tag{27}
\end{aligned}$$

where the last inequality uses

$$\begin{aligned}
\left| \frac{\mu_j}{p} + \frac{1}{n} \sum_{i=1}^n \varepsilon_{ji} \right| &\stackrel{\varepsilon}{\geq} \frac{\mu_j}{p} - 2(1 + \kappa_1) \sqrt{\frac{\mu_j \log M}{npN}} \\
&= \frac{\mu_j}{p} \left( 1 - 2(1 + \kappa_1) \sqrt{\frac{p \log M}{\mu_j n N}} \right) \\
&\stackrel{(13)}{\geq} \frac{\mu_j}{p} \left( 1 - 2(1 + \kappa_1) \sqrt{\frac{3}{2n}} \right) = \frac{\mu_j}{p} (1 - \kappa_1(1 + \kappa_1))
\end{aligned}$$

by recalling that  $\kappa_1 = \sqrt{6/n}$ . Since

$$(D_\Pi^{-1})_{jj} = \frac{1}{\sum_{i=1}^n (AW)_{ji}} = \frac{1}{\sum_{i=1}^n \Pi_{ji}} = \frac{p}{n\mu_j}, \tag{28}$$

combined with (27), we find

$$\begin{aligned}
n \left| (D_X^{-1})_{jj} \right| &\leq \frac{p}{\mu_j} \left( 1 + \frac{2(1 + \kappa_1)}{1 - \kappa_1(1 + \kappa_1)} \sqrt{\frac{p \log M}{\mu_j n N}} \right) \\
&\stackrel{(13)}{\leq} \left( 1 + \frac{\kappa_1(1 + \kappa_1)}{1 - \kappa_1(1 + \kappa_1)} \right) \frac{p}{\mu_j} \\
&= \frac{1}{1 - \kappa_1(1 + \kappa_1)} \cdot \frac{p}{\mu_j} \tag{29}
\end{aligned}$$

Finally, since  $|\widehat{\Theta}_{j\ell}| \leq \Theta_{j\ell} + |\widehat{\Theta}_{j\ell} - \Theta_{j\ell}|$ , combining (28) and (29) gives

$$\begin{aligned}
|T_4| + |T_5| &\leq \frac{2(1 + \kappa_1)}{(1 - \kappa_1(1 + \kappa_1))^2} \cdot \frac{p^2}{\mu_j \mu_\ell} \left( \sqrt{\frac{p}{\mu_j}} + \sqrt{\frac{p}{\mu_\ell}} \right) \sqrt{\frac{\log M}{nN}} \left( \Theta_{j\ell} + |\widehat{\Theta}_{j\ell} - \Theta_{j\ell}| \right), \\
|T_6| &= \frac{p^2}{\mu_j \mu_\ell} |\widehat{\Theta}_{j\ell} - \Theta_{j\ell}|.
\end{aligned}$$

Collecting these bounds for  $T_4$ ,  $T_5$  and  $T_6$  and using (13) again yield

$$|(\widehat{R} - R)_{j\ell}| \leq (1 + \kappa_1 \kappa_3) \frac{p^2}{\mu_j \mu_\ell} |\widehat{\Theta}_{j\ell} - \Theta_{j\ell}| + \kappa_3 \frac{p^2 \Theta_{j\ell}}{\mu_j \mu_\ell} \left( \sqrt{\frac{p}{\mu_j}} + \sqrt{\frac{p}{\mu_\ell}} \right) \sqrt{\frac{\log M}{nN}}.$$

with

$$\kappa_3 = \frac{2(1 + \kappa_1)}{(1 - \kappa_1 - \kappa_1^2)^2}.$$

This completes the proof of Proposition 8.  $\square$

**Proof of Corollary 9.** It suffices to show the following on the event  $\mathcal{E}$ ,

$$|\widehat{\Theta}_{j\ell} - \Theta_{j\ell}| = O\left(\sqrt{\frac{\log M}{nN}}\right), \quad \frac{|\widehat{m}_j - m_j|}{p} = O\left(\sqrt{\frac{\log M}{N}}\right), \quad \frac{|\widehat{\mu}_j - \mu_j|}{p} = O\left(\sqrt{\frac{\log M}{nN}}\right),$$

for all  $j, \ell \in [p]$ . Recall that the definitions (2). Since

$$\frac{\mu_j}{p} = \frac{1}{n} \sum_{i=1}^n \Pi_{ji} \leq \max_{1 \leq i \leq n} \Pi_{ji} = \frac{m_j}{p} \leq 1, \quad \Theta_{j\ell} = \frac{1}{n} \sum_{i=1}^n \Pi_{ji} \Pi_{\ell i} \leq 1, \quad (30)$$

for any  $j, \ell \in [p]$ , display (17) implies

$$\eta_{j\ell} \leq 3\sqrt{\frac{6 \log M}{nN}} + \frac{2 \log M}{nN} + 31(1 + \kappa_1) \sqrt{\frac{2(\log M)^4}{nN^3}} + \kappa_2 = O(\sqrt{\log M/(nN)}).$$

In addition,

$$\begin{aligned} \frac{|\widehat{\mu}_j - \mu_j|}{p} &= \frac{1}{n} \left| \sum_{i=1}^n (X_{ji} - \Pi_{ji}) \right| = \frac{1}{n} \left| \sum_{i=1}^n \varepsilon_{ji} \right| \\ &\stackrel{\mathcal{E}}{\leq} 2(1 + \kappa_1) \sqrt{\frac{\mu_j \log M}{npN}} \\ &\stackrel{(30)}{\leq} 2(1 + \kappa_1) \sqrt{\frac{\log M}{nN}} = O\left(\sqrt{\frac{\log M}{nN}}\right). \end{aligned}$$

Finally, we show  $|\widehat{m}_j - m_j|/p = O(\sqrt{\log M/N})$ . Fix any  $j \in [p]$  and define

$$i^* := \operatorname{argmax}_{1 \leq i \leq n} \Pi_{ji}, \quad i' := \operatorname{argmax}_{1 \leq i \leq n} X_{ji}.$$

Thus, from the definitions (2) and (21), we have

$$\begin{aligned} \frac{|\widehat{m}_j - m_j|}{p} &= |X_{ji'} - \Pi_{ji^*}| \\ &\leq |X_{ji'} - \Pi_{ji'}| + |\Pi_{ji^*} - \Pi_{ji'}| \\ &\leq 2|X_{ji'} - \Pi_{ji'}| + |X_{ji^*} - M_{ji^*}| + X_{ji^*} - X_{ji'} \\ &\leq 2|\varepsilon_{ji'}| + |\varepsilon_{ji^*}|, \end{aligned}$$

from the definition of  $i'$ .

From the proof of Lemma 7, we conclude, on the event  $\mathcal{S}_{ji}$ , that holds with probability at least  $1 - 2M^{-3}$ ,

$$\frac{|\hat{m}_j - m_j|}{p} \leq 2|\varepsilon_{ji'}| + |\varepsilon_{ji^*}| \stackrel{\mathcal{S}_{ji}}{\leq} 3\sqrt{\frac{6\Pi_{ji^*} \log M}{N}} + \frac{6 \log M}{N} \stackrel{(30)}{=} O\left(\sqrt{\frac{\log M}{N}}\right).$$

This completes the proof.  $\square$

The following corollary provides the expressions of  $\delta_{j\ell}$  and  $\eta_{j\ell}$  under condition (27).

**Corollary 10.** *Under model (3) and (27), with probability greater than  $1 - O(M^{-1})$ ,*

$$|\hat{\Theta}_{j\ell} - \Theta_{j\ell}| \leq c_0 \eta_{j\ell}, \quad |\hat{R}_{j\ell} - R_{j\ell}| \leq c_1 \delta_{j\ell}, \quad \text{for all } 1 \leq j, \ell \leq p$$

for some constant  $c_0, c_1 > 0$ , where

$$\begin{aligned} \eta_{j\ell} = & \sqrt{\frac{\Theta_{j\ell} \log M}{nN}} \sqrt{\frac{m_j + m_\ell}{p} \vee \frac{\log^2 M}{N}} + \frac{2(m_j + m_\ell) \log M}{p} \frac{1}{nN} \\ & + \sqrt{\frac{\log^4 M}{nN^3}} \sqrt{\frac{\mu_j + \mu_\ell}{p} \vee \frac{\log M}{N}} \end{aligned} \quad (31)$$

and

$$\delta_{j\ell} := \frac{p^2 \eta_{j\ell}}{\mu_j \mu_\ell} + \frac{p^2 \Theta_{j\ell}}{\mu_j \mu_\ell} \left( \sqrt{\frac{p}{\mu_j}} + \sqrt{\frac{p}{\mu_\ell}} \right) \sqrt{\frac{\log M}{nN}}. \quad (32)$$

**Proof.** We define the event  $\mathcal{E}' := \mathcal{E}'_1 \cap \mathcal{E}_2 \cap \mathcal{E}'_3$  with

$$\begin{aligned} \mathcal{E}'_1 = & \bigcap_{j=1}^p \left\{ \frac{1}{n} \left| \sum_{i=1}^n \varepsilon_{ji} \right| \lesssim \sqrt{\frac{\mu_j \log M}{npN}} \right\}, \\ \mathcal{E}_2 = & \bigcap_{j,\ell=1}^p \left\{ \frac{1}{n} \left| \sum_{i=1}^n \Pi_{\ell i} \varepsilon_{ji} \right| \leq \sqrt{\frac{6m_\ell \Theta_{j\ell} \log M}{npN}} + \frac{2m_\ell \log M}{npN} \right\}, \\ \mathcal{E}'_3 = & \bigcap_{j,\ell=1}^p \left\{ \frac{1}{n} \left| \sum_{i=1}^n (\varepsilon_{ji} \varepsilon_{\ell i} - \mathbb{E}[\varepsilon_{ji} \varepsilon_{\ell i}]) \right| \lesssim \sqrt{\frac{\Theta_{j\ell} \log^3 M}{nN^2}} + \sqrt{\frac{\log^5 M}{nN^4}} \right. \\ & \left. + \sqrt{\frac{(\mu_j + \mu_\ell) \log^4 M}{npN^3}} \right\}. \end{aligned}$$

From display (8) in the proof of Lemma 5 and condition (27), one has  $\mathbb{P}(\mathcal{E}'_1) \geq 1 - O(M^{-1})$ . Further invoking Lemma 6 and (9) – (11) in Lemma 7 yields  $\mathbb{P}(\mathcal{E}') \geq 1 - O(M^{-1})$ .

We proceed to work on  $\mathcal{E}'$ . The bound of  $|\hat{\Theta}_{j\ell} - \Theta_{j\ell}|$  requires upper bounds of  $T_1$ ,  $T_2$  and  $T_3$  defined in (22). From (23) – (25) and by invoking  $\mathcal{E}'$ , after a bit algebra, we have

$$\begin{aligned} |\hat{\Theta}_{j\ell} - \Theta_{j\ell}| &\lesssim \sqrt{\frac{\Theta_{j\ell} \log M}{nN}} \sqrt{\frac{\log^2 M}{N} \vee \frac{m_j + m_\ell}{p}} + \frac{(m_j + m_\ell) \log M}{npN} \\ &\quad + \sqrt{\frac{\log^4 M}{nN^3}} \sqrt{\frac{\log M}{N} \vee \frac{\mu_j + \mu_\ell}{p}}. \end{aligned}$$

Finally, the bound of  $|\hat{R}_{j\ell} - R_{j\ell}|$  follows from the same arguments in the proof of Proposition 8 by invoking condition (27) instead of (13).  $\square$

### C.3. Proofs of Theorem 4

We start by stating and proving the following lemma which is crucial for the proof of Theorem 4. Recall

$$J_1^a := \{j \in [p] : \tilde{A}_{ja} \geq 1 - 4\delta/\nu\}, \quad \text{for all } a \in [K].$$

Let

$$\hat{a}_i = \operatorname{argmax}_{1 \leq j \leq p} \hat{R}_{ij}, \quad \text{for any } i \in [p].$$

**Lemma 11.** *Under the conditions in Theorem 4, for any  $i \in I_a$  with some  $a \in [K]$ , the following inequalities hold on the event  $\mathcal{E}$ :*

$$|\hat{R}_{ij} - \hat{R}_{ik}| \leq \delta_{ij} + \delta_{ik}, \quad \text{for all } j, k \in I_a; \quad (33)$$

$$\hat{R}_{ij} - \hat{R}_{ik} > \delta_{ij} + \delta_{ik}, \quad \text{for all } j \in I_a, k \notin I_a \cup J_1^a; \quad (34)$$

$$\hat{R}_{ij} - \hat{R}_{ik} < \delta_{ij} + \delta_{ik}, \quad \text{for all } j \in J_1^a \text{ and } k \in I_a. \quad (35)$$

For any  $i \in J_1^a$ , we have

$$\hat{R}_{i\hat{a}_i} - \hat{R}_{ij} \leq \delta_{i\hat{a}_i} + \delta_{ij}, \quad \text{for any } j \in I_a. \quad (36)$$

**Proof.** We work on the event  $\mathcal{E}$  so that, in particular,  $|\hat{R}_{j\ell} - R_{j\ell}| \leq \delta_{j\ell}$  for all  $1 \leq j, \ell \leq p$ . To prove (33), fix  $i \in I_a$  and  $j, k \in I_a$  with some  $a \in [K]$ . Since  $R = \tilde{A}\tilde{C}\tilde{A}^T$ , we have  $R_{ij} = R_{ik} = \tilde{C}_{aa}$  and

$$|\hat{R}_{ij} - \hat{R}_{ik}| \leq |\hat{R}_{ij} - R_{ij}| + |\hat{R}_{ik} - R_{ik}| \stackrel{\mathcal{E}}{\leq} \delta_{ij} + \delta_{ik}.$$

To prove (34), fix  $i, j \in I_a$  and  $k \in [p] \setminus I_a$ . On the one hand,

$$\hat{R}_{ik} \stackrel{\mathcal{E}}{\leq} \sum_{b=1}^K \tilde{A}_{kb} \tilde{C}_{ab} + \delta_{ik} \stackrel{(23)}{\leq} \tilde{A}_{ka} \tilde{C}_{aa} + (1 - \tilde{A}_{ka})(\tilde{C}_{aa} - \nu) + \delta_{ik} = \tilde{C}_{aa} - (1 - \tilde{A}_{ka})\nu + \delta_{ik}. \quad (37)$$

On the other hand,  $i, j \in I_a$  implies  $R_{ij} = \tilde{C}_{aa}$ . Thus, on the event  $\mathcal{E}$ , (37) gives

$$\hat{R}_{ij} - \hat{R}_{ik} \stackrel{\mathcal{E}}{\geq} (1 - \tilde{A}_{ka})\nu - \delta_{ij} - \delta_{ik}.$$

If  $\tilde{A}_{ka} = 0$ , using (24) and  $\nu > 4\delta$  gives the desired result. If  $\tilde{A}_{ka} > 0$ , from the definition of  $J_1^a$ , we have  $\tilde{A}_{ka} < 1 - 4\delta/\nu$  which finishes the proof by using (24) again.

To prove (35), observe that, for any  $j \in J_1^a$  and  $k \in I_a$ ,

$$\hat{R}_{ij} \stackrel{(37)}{\leq} \tilde{C}_{aa} - (1 - \tilde{A}_{ja})\nu + \delta_{ij} < \tilde{C}_{aa} + \delta_{ij} = R_{ik} + \delta_{ij} \stackrel{\mathcal{E}}{\leq} \hat{R}_{ik} + \delta_{ij} + \delta_{ik}.$$

It remains to show (36). For any  $i \in J_1^a$  and  $j \in I_a$ , we have, for some  $c \in [K]$ ,

$$\begin{aligned} \hat{R}_{i\hat{a}_i} &\stackrel{\mathcal{E}}{\leq} \max_{k \in [p]} R_{ik} + \delta_{i\hat{a}_i} \stackrel{(*)}{\leq} \sum_{b=1}^K \tilde{A}_{ib} \tilde{C}_{bc} + \delta_{i\hat{a}_i} \\ &\stackrel{(**)}{\leq} \sum_{b=1}^K \tilde{A}_{ib} \tilde{C}_{ba} + \delta_{i\hat{a}_i} \\ &= R_{ij} + \delta_{i\hat{a}_i} \stackrel{\mathcal{E}}{\leq} \hat{R}_{ij} + \delta_{ij} + \delta_{i\hat{a}_i}. \end{aligned}$$

Inequality (\*) holds since

$$\max_{k \in [p]} R_{ik} = \max_{k \in [p]} \sum_{b=1}^K \tilde{A}_{kb} \left( \sum_{a=1}^K \tilde{A}_{ia} \tilde{C}_{ab} \right) \leq \max_{k \in [p]} \max_{b \in [K]} \sum_{a=1}^K \tilde{A}_{ia} \tilde{C}_{ab} = \sum_{a=1}^K \tilde{A}_{ia} \tilde{C}_{ac}.$$

Inequality (\*\*) holds, since, for any  $c \neq a$ , we have

$$\sum_{b=1}^K \tilde{A}_{ib} \tilde{C}_{bc} \leq \tilde{A}_{ia} \tilde{C}_{ac} + (1 - \tilde{A}_{ia}) \tilde{C}_{cc} \stackrel{(23)}{\leq} \tilde{A}_{ia} (\tilde{C}_{aa} - \nu) + (1 - \tilde{A}_{ia}) \tilde{C}_{cc},$$

and

$$\sum_{b=1}^K \tilde{A}_{ib} \tilde{C}_{ab} \stackrel{(23)}{\geq} \tilde{A}_{ia} \tilde{C}_{aa}.$$

$$\sum_{b=1}^K \tilde{A}_{ib} \tilde{C}_{ab} - \sum_{b=1}^K \tilde{A}_{ib} \tilde{C}_{bc} \geq \tilde{A}_{ia} \nu - (1 - \tilde{A}_{ia}) \tilde{C}_{cc} > \nu - 2(1 - \tilde{A}_{ia}) \tilde{C}_{cc}.$$

The term on the right is positive, since condition (25) guarantees that

$$\nu \geq \frac{8\delta}{\nu} \tilde{C}_{cc} \geq 2(1 - \tilde{A}_{ia}) \tilde{C}_{cc},$$

where the last inequality is due to the definition of  $J_1$ . This concludes the proof.  $\square$

Lemma 11 remains valid under the conditions of Corollary 5 in which case  $J_1 = \emptyset$  and we only need  $\nu > 4\delta$  to prove (34).

**Proof of Theorem 4.** We work on the event  $\mathcal{E}$  throughout the proof. Without loss of generality, we assume that the label permutation  $\pi$  is the identity. We start by presenting three claims which are sufficient to prove the result. Let  $\hat{I}^{(i)}$  be defined in step 5 of Algorithm 2 for any  $i \in [p]$ .

- (1) For any  $i \in J \setminus J_1$ , we have  $\hat{I}^{(i)} \notin \hat{\mathcal{I}}$ .
- (2) For any  $i \in I_a$  and  $a \in [K]$ , we have  $i \in \hat{I}^{(i)}$ ,  $I_a \subseteq \hat{I}^{(i)}$  and  $\hat{I}^{(i)} \setminus I_a \subseteq J_1^a$ .
- (3) For any  $i \in J_1^a$  and  $a \in [K]$ , we have  $I_a \subseteq \hat{I}^{(i)}$ .

If we can prove these claims, then (1) and the MERGE step in Algorithm 2 guarantees that  $\hat{I} \cap (J \setminus J_1) = \emptyset$  and thus enable us to focus on  $i \in I \cap J_1$ . For any  $a \in [K]$ , (2) implies that there exists  $i \in I_a$  such that  $I_a \subseteq \hat{I}^{(i)}$  and  $\hat{I}^{(i)} \setminus I_a \subseteq J_1^a$  with  $\hat{I}^{(i)} := \hat{I}_a$ . Finally, (3) guarantees that none of anchor words will be excluded by any  $i \in J_1$  in the MERGE step. Thus,  $\hat{K} = K$  and  $\hat{\mathcal{I}} = \{\hat{I}_1, \dots, \hat{I}_K\}$  is the desired partition. Therefore, we proceed to prove (1) - (3) in the following. Recall that  $\hat{a}_i := \arg\max_{1 \leq j \leq p} \hat{R}_{ij}$  for all  $1 \leq i \leq p$ .

To prove (1), let  $i \in J \setminus J_1$  be fixed. We first prove that  $\hat{I}^{(i)} \notin \hat{\mathcal{I}}$  when  $\hat{I}^{(i)} \cap I \neq \emptyset$ . From steps 8 - 10 of Algorithm 2, it suffices to show that, there exists  $j \in \hat{I}^{(i)}$  such that the following does not hold for any  $k \in \hat{a}_j$ :

$$|\hat{R}_{ij} - \hat{R}_{jk}| \leq \delta_{ij} + \delta_{jk}. \quad (38)$$

Let  $\hat{I}^{(i)} \cap I \neq \emptyset$  such that there exists  $j \in I_b \cap \hat{I}^{(i)}$  for some  $b \in [K]$ . For this  $j$ , we have  $R_{ij} = \sum_a \tilde{A}_{ia} \tilde{C}_{ab}$  and

$$\hat{R}_{ij} \stackrel{(37)}{\leq} \tilde{C}_{bb} - (1 - \tilde{A}_{ib})\nu + \delta_{ij}. \quad (39)$$

On the other hand, for any  $k \in \hat{a}_j$  and  $k' \in I_b$ , using the definition of  $\hat{a}_j$  gives

$$\hat{R}_{jk} \geq \hat{R}_{jk'} \stackrel{\mathcal{E}}{\geq} R_{jk'} + \delta_{jk'} = \tilde{C}_{bb} - \delta_{jk'}. \quad (40)$$

Combining (39) with (40) gives

$$\hat{R}_{jk} - \hat{R}_{ij} \geq (1 - \tilde{A}_{ib})\nu - \delta_{ij} - \delta_{jk'}.$$

The definition of  $J_1$  and (24) with  $\nu > 4\delta$  give

$$\hat{R}_{jk} - \hat{R}_{ij} > \delta_{jk} + \delta_{ij}.$$

This shows that for any  $i \in J \setminus J_1$ , if  $\hat{I}^{(i)} \cap I \neq \emptyset$ ,  $\hat{I}^{(i)} \notin \hat{\mathcal{I}}$ . Therefore, to complete the proof of (1), we show that  $\hat{I}^{(i)} \cap I = \emptyset$  is impossible if  $i \in J \setminus J_1$ . For fixed  $i \in J \setminus J_1$  and  $j \in \hat{a}_i$ , we have

$$R_{ij} = \sum_b \sum_a \tilde{A}_{ia} \tilde{A}_{jb} \tilde{C}_{ab} \leq \max_{1 \leq b \leq K} \sum_a \tilde{A}_{ia} \tilde{C}_{ab} = \sum_a \tilde{A}_{ia} \tilde{C}_{ab^*} = R_{ik}$$

for some  $b^*$  and any  $k \in I_{b^*}$ . Therefore,

$$\widehat{R}_{ij} - \widehat{R}_{ik} \stackrel{\varepsilon}{\leq} R_{ij} - R_{ik} + \delta_{ij} + \delta_{ik} \leq \delta_{ij} + \delta_{ik}$$

On the other hand, assume  $\widehat{I}^{(i)} \cap I = \emptyset$ . Since  $k \in I_{b^*}$ , we know  $k \notin \widehat{I}^{(i)}$ , which implies

$$\widehat{R}_{ij} - \widehat{R}_{ik} > \delta_{ij} + \delta_{ik},$$

from step 5 of Algorithm 2. The last two displays contradict each other, and we conclude that, for any  $i \in J \setminus J_1$ ,  $\widehat{I}^{(i)} \cap I \neq \emptyset$ . This completes the proof of (1).

From (34) in Lemma 11, given step 5 of Algorithm 2, we know that, for any  $j \in \widehat{I}^{(i)}$ ,  $j \in I_a \cup J_1^a$ . Thus, we write  $\widehat{I}^{(i)} = (\widehat{I}^{(i)} \cap I_a) \cup (\widehat{I}^{(i)} \cap J_1^a)$ . For any  $j \in \widehat{I}^{(i)} \cap I_a$ , by the same reasoning,  $\widehat{a}_j$  is either  $I_a$  or  $J_1^a$ . For both cases, since  $i, j \in I_a$  and  $i \neq j$ , (33) and (36) in Lemma 11 guarantee that (38) holds. On the other hand, for any  $j \in \widehat{I}^{(i)} \cap J_1^a$ , (35) in Lemma 11 implies that (38) still holds. Thus, we have shown that, for any  $i \in I_a$ ,  $i \in \widehat{I}^{(i)}$ . To show  $I_a \subseteq \widehat{I}^{(i)}$ , let any  $j \in I_a$  and observe that  $\widehat{a}_i$  can only be in  $I_a \cup J_1^a$ . In both cases, (33) and (36) imply  $j \in \widehat{I}^{(i)}$ . Thus,  $I_a \subseteq \widehat{I}^{(i)}$ . Finally,  $\widehat{I}^{(i)} \setminus I_a \subseteq J_1^a$  follows immediately from (34).

We conclude the proof by noting that (3) directly follows from (35).  $\square$

## Appendix D: Proofs of Section 5

### D.1. Proofs of Lower bounds in Section 5.1

**Proof of Theorem 6.** We first show the result of the matrix  $\ell_1$  norm. Let

$$A^{(0)} = \begin{bmatrix} e_1 \otimes \mathbf{1}_{g_1} & e_2 \otimes \mathbf{1}_{g_2} & \cdots & e_K \otimes \mathbf{1}_{g_K} \\ \mathbf{1}_{|J|} & \mathbf{1}_{|J|} & \cdots & \mathbf{1}_{|J|} \end{bmatrix} \times \begin{bmatrix} \frac{1}{g_1 + |J|} & & & \\ & \ddots & & \\ & & \ddots & \\ & & & \frac{1}{g_K + |J|} \end{bmatrix} \quad (41)$$

with  $g_k := |I_k|$  for any  $1 \leq k \leq K$  and  $|g_k - g_{k+1}| \leq 1$ . We use  $e_k$  to denote the canonical basis vectors in  $\mathbb{R}^K$  and use  $\mathbf{1}_d$  and  $\otimes$  to denote, respectively, the  $d$ -dimensional vector with entries equal to 1 and the kronecker product. We start by constructing a set of “hypotheses” of  $A$ . Assume  $g_k + |J|$  is even for  $1 \leq k \leq K$ . Let

$$M := \{0, 1\}^{(|I| + |J|K)/2}.$$

Following the Varshamov-Gilbert bound in Lemma 2.9 in [6], there exists  $w^{(j)} \in M$  for  $j = 0, 1, \dots, T$ , such that

$$\|w^{(i)} - w^{(j)}\|_1 \geq \frac{|I| + K|J|}{16}, \quad \text{for any } 0 \leq i \neq j \leq T, \quad (42)$$

with  $w^{(0)} = 0$  and

$$\log(T) \geq \frac{\log(2)}{16}(|I| + K|J|). \quad (43)$$

For each  $w^{(j)} \in \mathbb{R}^{(|I|+K|J|)/2}$ , we divide it into  $K$  chunks as  $w^{(j)} = (w_1^{(j)}, w_2^{(j)}, \dots, w_K^{(j)})$  with  $w_k^{(j)} \in \mathbb{R}^{(g_k+|J|)/2}$ . For each  $w_k^{(j)}$ , we write  $\tilde{w}_k^{(j)} \in \mathbb{R}^p$  as its augmented counterpart such that  $\tilde{w}_k^{(j)}(S_k) = [w_k^{(j)}, -w_k^{(j)}]$  and  $\tilde{w}_k^{(j)}(\ell) = 0$  for any  $\ell \notin S_k$ , where  $S_k := \text{supp}(A_k^{(0)})$ . For  $1 \leq j \leq T$ , we choose  $A^{(j)}$  as

$$A^{(j)} = A^{(0)} + \gamma \begin{bmatrix} \tilde{w}_1^{(j)} & \dots & \tilde{w}_K^{(j)} \end{bmatrix} \quad (44)$$

with

$$\gamma = \sqrt{\frac{\log(2)}{16^2 c^2 (1 + c_0)}} \sqrt{\frac{K^2}{nN(|I| + K|J|)}} \quad (45)$$

for some constant  $c_0, c > 0$ . Under  $|I| + K|J| \leq c(nN)$ , it is easy to verify that  $A^{(j)} \in \mathcal{A}(K, |I|, |J|)$  for all  $0 \leq j \leq T$ .

In order to apply Theorem 2.5 in [6], we need to check the following conditions:

- (a)  $\text{KL}(\mathbb{P}_{A^{(j)}}, \mathbb{P}_{A^{(0)}}) \leq \log(T)/16$ , for each  $i = 1, \dots, T$ .
- (b)  $L_1(A^{(i)}, A^{(j)}) \geq c_1 K \sqrt{(|I| + K|J|)/(nN)}$ , for  $0 \leq i < j \leq T$  and some positive constant  $c_1$ .
- (c)  $L_1(\cdot)$  satisfies the triangle inequality.

The expression of Kullback-Leibler divergence between two multinomial distributions is shown in [3, Lemma 6.7]. For completeness, we include it here.

**Lemma 12** (Lemma 6.7 [3]). *Let  $D$  and  $D'$  be two  $p \times n$  matrices such that each column of them is a weight vector. Under model (3), let  $\mathbb{P}$  and  $\mathbb{P}'$  be the probability measures associated with  $D$  and  $D'$ , respectively. Suppose  $D$  is a positive matrix. Let*

$$\eta = \max_{1 \leq j \leq p, 1 \leq i \leq n} \frac{|D'_{ji} - D_{ji}|}{D_{ji}}$$

and assume  $\eta < 1$ . There exists a universal constant  $c_0 > 0$  such that

$$\text{KL}(\mathbb{P}', \mathbb{P}) \leq (1 + c_0 \eta) N \sum_{i=1}^n \sum_{j=1}^p \frac{|D'_{ji} - D_{ji}|^2}{D_{ji}}.$$

Fix  $1 \leq j \leq T$  and choose  $D^{(j)} = A^{(j)}W$  with

$$W \in \mathbb{R}_+^{K \times n} = W^0 + \frac{1}{nN} \mathbf{1}_K \mathbf{1}_K^T - \frac{K}{nN} \mathbf{I}_K$$

where  $W^0$  is defined in (35). The above choice of  $W$  perturbs  $W^0$  to avoid  $D_{ji} \neq 0$  for any  $j \in I$  and  $i \in [n]$ , in the presence of anchor words. Since there exists some large enough constant  $c > 0$  such that  $g_k \leq c|I|/K$ , it then follows that

$$D_{\ell i}^{(0)} = \sum_{k=1}^K A_{\ell k}^{(0)} W_{ki} = \begin{cases} W_{ki}/(g_k + |J|) \geq cW_{ki}/(|I|/K + |J|) & \text{if } \ell \in I_k, k \in [K] \\ \sum_k W_{ki}/(g_k + |J|) \geq c/(|I|/K + |J|) & \text{if } \ell \in J \end{cases} \quad (46)$$

for any  $1 \leq i \leq n$ , where we also use  $\sum_k W_{ki} = 1$ . Similarly, we have

$$\left| D_{\ell i}^{(j)} - D_{\ell i}^{(0)} \right| = \gamma \left| \sum_{k=1}^K \tilde{w}_k^{(j)}(\ell) W_{ki} \right| \leq \begin{cases} W_{ki}\gamma & \text{if } \ell \in I_k, k \in [K] \\ \gamma & \text{if } \ell \in J \end{cases} \quad (47)$$

for all  $1 \leq i \leq n$ , where  $\tilde{w}_k^{(j)}(\ell)$  denotes the  $\ell$ th element of  $\tilde{w}_k^{(j)}$ . Thus, by choosing proper  $c_0$  in (45) and using  $|I| + K|J| \leq c(nN)$ , we have

$$\max_{1 \leq \ell \leq p, 1 \leq i \leq n} \frac{|D_{\ell i}^{(j)} - D_{\ell i}^{(0)}|}{D_{\ell i}^{(0)}} \leq c\gamma(|I|/K + |J|) < 1,$$

for any  $1 \leq j \leq T$ . Invoking Lemma 12 gives

$$\begin{aligned} \text{KL}(\mathbb{P}_{A^{(j)}}, \mathbb{P}_{A^{(0)}}) &\leq (1 + c_0) N \sum_{i=1}^n \sum_{\ell=1}^p \frac{|D_{\ell i}^{(j)} - D_{\ell i}^{(0)}|^2}{D_{\ell i}^{(0)}} \\ &\leq c(1 + c_0) N \left( \frac{|I|}{K} + |J| \right) \sum_{i=1}^n \left\{ \gamma^2 |J| + \sum_{k=1}^K \gamma^2 g_k W_{ki} \right\} \\ &\leq c(1 + c_0) nN (|I| + K|J|)^2 \gamma^2 / K^2 \\ &\stackrel{(43)}{\leq} \frac{1}{16} \log T, \end{aligned}$$

where the second inequality uses (46) and (47) and the third inequality uses  $g_k \leq c|I|/K$  and  $\sum_k W_{ki} = 1$ . This verifies (a).

To show (b), from (44), it gives

$$\begin{aligned} L_1(A^{(j)}, A^{(\ell)}) &= \sum_{k=1}^K \left\| A_{\cdot k}^{(j)} - A_{\cdot k}^{(\ell)} \right\|_1 \\ &= 2\gamma \sum_{k=1}^K \left\| w_k^{(j)} - w_k^{(\ell)} \right\|_1 \\ &= 2\gamma \left\| w^{(j)} - w^{(\ell)} \right\|_1 \\ &\stackrel{(42)}{\geq} \frac{\gamma}{8} (|I| + K|J|). \end{aligned}$$

Plugging into the expression of  $\gamma$  verifies (b). Since (c) is already verified in [3, page 31], invoking [6, Theorem 2.5] concludes the proof for even  $g_k + |J|$ . The complementary case is easy to derive with slight modifications. Specifically, denote by  $\mathcal{S}_{odd} := \{1 \leq k \leq K : g_k + |J| \text{ is odd}\}$ . Then we change  $M := \{0, 1\}^{Card}$  with

$$Card = \sum_{k \in \mathcal{S}_{odd}} \frac{g_k + |J| - 1}{2} + \sum_{k \in \mathcal{S}_{odd}^c} \frac{g_k + |J|}{2}.$$

For each  $w^{(j)}$ , we write it as  $w^{(j)} = (w_1^{(j)}, \dots, w_K^{(j)})$  and each  $w_k^{(j)}$  has length  $(g_k + |J| - 1)/2$  if  $k \in \mathcal{S}_{odd}$  and  $(g_k + |J|)/2$  otherwise. We then construct  $A_k^{(j)} = A_k^{(0)} + \gamma \tilde{w}_k^{(j)}$  where  $\tilde{w}_k^{(j)} \in \mathbb{R}^p$  is the same augmented counterpart of  $w_k^{(j)}$ . The result follows from the same arguments.

To conclude the proof, we show the lower bound of  $\|\hat{A} - A\|_{1,\infty}$ . Let  $k^* := \arg \max_k g_k$ . Then we can repeat the above arguments by only changing the  $k^*$ th column of  $A^{(0)}$ . Specifically, assume  $|J| + g_{k^*}$  is even and we draw  $w^{(j)}$  from  $M = \{0, 1\}^{(|J| + g_{k^*})/2}$  for  $1 \leq j \leq T$  with

$$\log(T) \geq \log(2)(|J| + g_{k^*})/16.$$

Let  $\tilde{w}^{(j)}$  be its augmented counterpart and choose  $A_k^{(j)} = A_k^{(0)} + \gamma \tilde{w}^{(j)}$  with

$$\gamma = \sqrt{\frac{\log(2)}{16^2 c^2 (1 + c_0)}} \sqrt{\frac{K}{nN(g_{k^*} + |J|)}}$$

and  $\|w^{(j)} - w^{(\ell)}\|_1 \geq (g_{k^*} + |J|)/16$  for any  $0 \leq j \neq \ell \leq T$ . Then we need to check

- (a')  $\text{KL}(\mathbb{P}_{A^{(j)}}, \mathbb{P}_{A^{(0)}}) \leq \log(T)/16$ , for each  $i = 1, \dots, T$ .
- (b')  $L_{1,\infty}(A^{(i)}, A^{(j)}) \geq c_1 \sqrt{K(g_{k^*} + |J|)/(nN)}$ , for  $0 \leq i < j \leq T$  and some positive constant  $c_1$ .
- (c')  $L_{1,\infty}(\cdot)$  satisfies the triangle inequality.

Different from (46) and (47), we have, for all  $1 \leq i \leq n$ ,

$$D_{\ell i}^{(0)} = \sum_{k=1}^K A_{\ell k}^{(0)} W_{ki} = \begin{cases} W_{ki}/(g_k + |J|) \geq W_{ki}/(g_{k^*} + |J|) & \text{if } \ell \in I_k, k \in [K] \\ \sum_k W_{ki}/(g_k + |J|) \geq 1/(g_{k^*} + |J|) & \text{if } \ell \in J \end{cases} \quad (48)$$

and

$$\left| D_{\ell i}^{(j)} - D_{\ell i}^{(0)} \right| = \begin{cases} \gamma W_{k^* i} \tilde{w}_\ell^{(j)} \leq \gamma W_{k^* i}, & \text{if } \ell \in I_{k^*} \cup J \\ 0, & \text{otherwise.} \end{cases} \quad (49)$$

Using the same arguments, one can derive

$$\text{KL}(\mathbb{P}_{A^{(j)}}, \mathbb{P}_{A^{(0)}}) \leq (1 + c_0) N \gamma^2 (g_{k^*} + |J|) \sum_{i=1}^n (W_{k^* i}^2 |J| + W_{k^* i} g_{k^*}).$$

Since there exists some constant  $c > 0$  such that

$$\sum_{i=1}^n (W_{k^*i}^2 |J| + W_{k^*i} g_{k^*}) = \sum_{a=1}^n \sum_{i \in n_a} (W_{k^*i}^2 |J| + W_{k^*i} g_{k^*}) \leq c(|J| + g_{k^*})n/K,$$

we conclude that

$$\text{KL}(\mathbb{P}_{A^{(j)}}, \mathbb{P}_{A^{(0)}}) \leq c(1 + c_0)\gamma^2 N n (g_{k^*} + |J|)^2 / K \leq \log(T)/16.$$

To show (b'), observe that

$$L_{1,\infty}(A^{(j)}, A^{(\ell)}) = 2\gamma \max_{1 \leq k \leq K} \|w_k^{(j)} - w_k^{(\ell)}\|_1 \geq \frac{\gamma(g_{k^*} + |J|)}{8}.$$

Finally, we verify (c') by showing that  $L_{1,\infty}(\cdot)$  satisfies the triangle inequality. Consider  $(A, \tilde{A}, \hat{A})$  and observe that

$$\begin{aligned} L_{1,\infty}(A, \tilde{A}) &= \min_{P \in \mathcal{H}_K} \|AP - \tilde{A}\|_{1,\infty} = \min_{P, Q \in \mathcal{H}_K} \|AP - \tilde{A}Q\|_{1,\infty} \\ &\leq \min_{P, Q \in \mathcal{H}_K} (\|AP - \hat{A}\|_{1,\infty} + \|\hat{A} - \tilde{A}Q\|_{1,\infty}) \\ &= \min_{P \in \mathcal{H}_K} \|AP - \hat{A}\|_{1,\infty} + \min_{Q \in \mathcal{H}_K} \|\hat{A} - \tilde{A}Q\|_{1,\infty} \\ &= L_{1,\infty}(A, \hat{A}) + L_{1,\infty}(\tilde{A}, \hat{A}). \end{aligned}$$

The proof is complete.  $\square$

## D.2. Proofs of upper bounds in Section 5.3

We work on the event  $\mathcal{E}$ . Recall that under (26), we have  $P(\mathcal{E}) \geq 1 - M^{-3}$ . From Theorem 4, we have  $\hat{K} = K$  and  $\hat{I} = I$ . Without loss of generality, we assume that the label permutation matrix  $\Pi$  is the identity matrix that aligns the topic words with the estimates ( $\hat{\mathcal{I}} = \mathcal{I}$ ). In particular, this implies that any chosen  $\hat{L} \subset I$  has the correct partition, and we have  $\hat{L} = L$ . We first give a crucial lemma to the proof of Theorem 7. From (17), recall that

$$\eta_{j\ell} \asymp (\sqrt{m_j} + \sqrt{m_\ell}) \sqrt{\frac{\Theta_{j\ell} \log M}{npN}} + \frac{(m_j + m_\ell) \log M}{npN} + \sqrt{\frac{(\mu_j + \mu_\ell)(\log M)^4}{npN^3}}, \quad (50)$$

for all  $j, \ell \in [p]$ .

**Lemma 13.** *Under the conditions of Theorem 7, we have*

$$\max_{i \in L} \sum_{j \in L} \eta_{ij} \lesssim \sqrt{\bar{\alpha}_I^3 \bar{\gamma}} \sqrt{\frac{\log M}{np^3 N}}, \quad (51)$$

$$\max_{i \in L} \sum_{j \in J} \eta_{ij} \lesssim \sqrt{\bar{\alpha}_I \bar{\gamma} S_J} \sqrt{\frac{\log M}{K np^2 N}}, \quad (52)$$

with  $S_J = |J|\bar{\alpha}_I + \sum_{j \in J} \alpha_j$ , for any  $i \in I_k$  and  $k \in [K]$ . In addition, if  $\sum_{k' \neq k} \sqrt{C_{kk'}} = o(\sqrt{C_{kk}})$  for any  $1 \leq k \leq K$ , then

$$\max_{i \in L} \sum_{j \in L} \eta_{ij} \lesssim \sqrt{\bar{\alpha}_I^3 \bar{\gamma}} \sqrt{\frac{\log M}{Knp^3N}}. \quad (53)$$

**Proof.** We first simplify the expression of  $\eta$  defined in (17). To show (51), observe that, for any  $i \in I_a$ ,  $j \in I_b$  and  $a, b \in [K]$ , we have

$$\Theta_{ij} = \frac{1}{n} \sum_{\ell=1}^n \Pi_{i\ell} \Pi_{j\ell} = A_{ia} A_{jb} \frac{1}{n} \sum_{\ell=1}^n W_{a\ell} W_{b\ell} \stackrel{(2)}{=} \frac{\alpha_i \alpha_j}{p^2} \cdot \frac{1}{n} \langle W_{a\cdot}, W_{b\cdot} \rangle.$$

As a result, plugging (14) - (16) and the above display into (17) yields

$$\eta_{ij} \asymp \sqrt{\frac{1}{n} \langle W_{a\cdot}, W_{b\cdot} \rangle} \sqrt{\frac{\bar{\alpha}_I^3 \log M}{np^3N}} + \frac{\bar{\alpha}_I \log M}{npN} + \sqrt{\frac{\bar{\alpha}_I \bar{\gamma} (\log M)^4}{KnpN^3}}. \quad (54)$$

Since

$$\sum_{b=1}^K \frac{1}{n} \langle W_{a\cdot}, W_{b\cdot} \rangle = \frac{1}{n} \sum_{\ell=1}^n W_{a\ell} \sum_{b=1}^K W_{b\ell} \stackrel{(1)}{=} \frac{1}{n} \sum_{\ell=1}^n W_{a\ell} \stackrel{(2)}{=} \frac{\gamma_a}{K},$$

summing (54) over  $j \in L$ , and using the Cauchy-Schwarz inequality to obtain the first term, gives

$$\max_{i \in L} \sum_{j \in L} \eta_{ij} \lesssim \sqrt{\frac{\bar{\alpha}_I \log M}{npN}} \left[ \sqrt{\frac{\bar{\alpha}_I^2 \bar{\gamma}}{p^2}} + \sqrt{\frac{\bar{\alpha}_I K^2 \log M}{npN}} + \sqrt{\frac{K \bar{\gamma} (\log M)^3}{N^2}} \right]. \quad (55)$$

Note that Assumption 2 implies  $n \geq K$ . Since (26) and (15) together with the fact  $\bar{\gamma} \geq 1 \geq \underline{\gamma}$  give

$$\frac{\bar{\alpha}_I \bar{\gamma}}{K} \geq \frac{\bar{\alpha}_I}{K} \geq \frac{\bar{\alpha}_I \underline{\gamma}}{K} \geq \min_{i \in I} \mu_i \geq \frac{2p \log M}{3N}, \quad (56)$$

these two bounds imply the first term on the right in (55) is greater than the second term on the right of (55). Moreover, (16), (26) and (56) imply

$$\frac{\bar{\alpha}_I^2}{Kp^2} \geq \frac{2 \log M}{3N} \frac{\bar{\alpha}_I}{p} \geq \frac{2 \log M}{3N} \frac{m_{\min}}{p} \geq \frac{6(\log M)^3}{N^2}.$$

Thus, the first term on the right of (55) is also greater than the third term on the right of (55). This finishes the proof of (51).

We proceed to show (52). For any  $i \in I_a$  and  $j \in [p]$ , observe that

$$\Theta_{ij} = \frac{1}{n} \sum_{\ell=1}^n \Pi_{i\ell} \Pi_{j\ell} = A_{ia} \frac{1}{n} \sum_{\ell=1}^n W_{a\ell} \Pi_{j\ell} \stackrel{(2)}{=} \frac{\alpha_i}{p} \cdot \frac{1}{n} \langle W_{a\cdot}, \Pi_{j\cdot} \rangle.$$

Plugging (14) – (16) and the above display into (17) yields

$$\eta_{ij} \lesssim \sqrt{\frac{1}{n} \langle W_{a\cdot}, \Pi_{j\cdot} \rangle} \sqrt{\frac{\alpha_i(\alpha_i + \alpha_j) \log M}{np^2 N}} + \frac{(\alpha_i + \alpha_j) \log M}{npN} + \sqrt{\frac{(\alpha_i + \alpha_j)(\log M)^4}{npN^3}}. \quad (57)$$

Since  $\sum_k W_{k\ell} = 1$  and (2) yield

$$\sum_{j \in J} \frac{1}{n} \langle W_{a\cdot}, \Pi_{j\cdot} \rangle = \sum_{k=1}^K \frac{1}{n} \sum_{\ell=1}^n W_{a\ell} W_{k\ell} \sum_{j \in J} A_{jk} \leq \frac{\gamma_a}{K} \|A_J\|_{1,\infty} \leq \frac{\gamma_a}{K},$$

summing (57) over  $j \in J$  and using Cauchy-Schwarz yield

$$\max_{i \in L} \sum_{j \in J} \eta_{ij} \lesssim \sqrt{\frac{S_J \log M}{npN}} \left( \sqrt{\frac{\bar{\alpha}_I \bar{\gamma}}{Kp}} + \sqrt{\frac{S_J \log M}{npN}} + \sqrt{\frac{|J|(\log M)^3}{N^2}} \right).$$

To conclude the proof of (52), it suffices to show the first term on the right in the display above dominates the other two. This is true by noting that

$$\frac{\bar{\alpha}_I \bar{\gamma} N^2}{K|J|p(\log M)^3} \geq \frac{\mu_{\min} N^2}{|J|p(\log M)^3} \gtrsim 1$$

and

$$\frac{\bar{\gamma} n N}{K|J| \log M} \gtrsim 1, \quad \frac{\bar{\alpha}_I \bar{\gamma} n N}{K \sum_{j \in J} \alpha_j \log M} \gtrsim 1$$

from the same arguments to prove (51) together with  $|J| \leq p$  and  $\sum_{j \in J} \alpha_j \leq Kp$ .

Finally, to show (53), invoking the additional condition and using (54) yield

$$\begin{aligned} \max_{i \in L} \sum_{j \in L} \eta_{ij} &\lesssim \max_{a \in [K]} \sqrt{C_{aa}} \sqrt{\frac{\bar{\alpha}_I^3 \log M}{np^3 N}} + \frac{K \bar{\alpha}_I \log M}{npN} + \sqrt{\frac{K \bar{\alpha}_I \bar{\gamma} (\log M)^4}{npN^3}} \\ &\leq \sqrt{\frac{\bar{\alpha}_I^3 \bar{\gamma} \log M}{K np^3 N}} + \frac{K \bar{\alpha}_I \log M}{npN} + \sqrt{\frac{K \bar{\alpha}_I \bar{\gamma} (\log M)^4}{npN^3}} \end{aligned}$$

where we use  $C_{aa} \leq n^{-1} \|W_{a\cdot}\|_1 \lesssim \bar{\gamma}/K$  to derive the second inequality. Repeating the same arguments, one can show that on the right-hand-side the first term dominates the second and third terms. This finishes the proof.  $\square$

#### D.2.1. Proof of Theorem 7

On the event  $\mathcal{E}$ , Theorem 4 guarantees that  $\hat{I} = I$ ,  $\hat{J} = J$  and  $\hat{L} = L$ . We work on this event for the remainder of the proof. Our proof consists of three parts for any  $k \in [K]$ : To obtain the error rate of (1)  $\|\hat{B}_{Ik} - B_{Ik}\|_1$ , (2)  $\|\hat{B}_{Jk} - B_{Jk}\|_1$  and (3)  $\|\hat{A}_{\cdot k} - A_{\cdot k}\|_1$ .

For step (1), recall (19) and (38). Then, for any  $1 \leq k \leq K$ , it follows

$$\|\hat{B}_{Ik} - B_{Ik}\|_1 = \sum_{i \in I_k} \left| \frac{\|X_{i\cdot}\|_1}{\|X_{i_k\cdot}\|_1} - \frac{\|\Pi_{i\cdot}\|_1}{\|\Pi_{i_k\cdot}\|_1} \right|$$

and we obtain

$$\begin{aligned} & \|\hat{B}_{Ik} - B_{Ik}\|_1 \\ &= \frac{1}{\|X_{i_k\cdot}\|_1 \|\Pi_{i_k\cdot}\|_1} \sum_{i \in I_k} \left| \|\Pi_{i_k\cdot}\|_1 \|X_{i\cdot}\|_1 - \|X_{i_k\cdot}\|_1 \|\Pi_{i\cdot}\|_1 \right| \\ &\leq \frac{1}{\|X_{i_k\cdot}\|_1 \|\Pi_{i_k\cdot}\|_1} \left[ \|\Pi_{i_k\cdot}\|_1 \sum_{i \in I_k} \left| \|X_{i\cdot}\|_1 - \|\Pi_{i\cdot}\|_1 \right| + \left| \|X_{i_k\cdot}\|_1 - \|\Pi_{i_k\cdot}\|_1 \right| \sum_{i \in I_k} \|\Pi_{i\cdot}\|_1 \right] \\ &= \frac{1}{\|X_{i_k\cdot}\|_1} \sum_{i \in I_k} \frac{1}{n} \left| \sum_{j=1}^n \varepsilon_{ij} \right| + \frac{\sum_{i \in I_k} \|\Pi_{i\cdot}\|_1}{\|X_{i_k\cdot}\|_1 \|\Pi_{i_k\cdot}\|_1} \frac{1}{n} \left| \sum_{j=1}^n \varepsilon_{i_k j} \right|. \end{aligned}$$

In the last step we used that  $X_i$  and  $\Pi_i$  have nonnegative entries only so that indeed

$$\begin{aligned} \left| \|X_{i\cdot}\|_1 - \|\Pi_{i\cdot}\|_1 \right| &= \frac{1}{n} \left| \sum_{j=1}^n |X_{ij}| - \sum_{j=1}^n |\Pi_{ij}| \right| \\ &= \frac{1}{n} \left| \sum_{j=1}^n X_{ij} - \sum_{j=1}^n \Pi_{ij} \right| \\ &= \frac{1}{n} \left| \sum_{j=1}^n \varepsilon_{ij} \right|. \end{aligned}$$

Invoking Lemma 5,  $n^{-1} \left| \sum_{j=1}^n \varepsilon_{ij} \right| \lesssim \sqrt{\mu_i p \log M / (nN)}$  on the event  $\mathcal{E}_1 \supset \mathcal{E}$ . Note further that, for any  $i \in [p]$ ,

$$\frac{1}{\|X_{i\cdot}\|_1} = (D_X)_{ii}^{-1} \stackrel{(29)}{\lesssim} \frac{p}{n\mu_i}$$

and  $\|\Pi_{i\cdot}\|_1 = n\mu_i/p$  by the definition in (2). Now deduce that

$$\|\hat{B}_{Ik} - B_{Ik}\|_1 \lesssim \frac{1}{\mu_{i_k}} \sum_{i \in I_k} \sqrt{\frac{\mu_i p \log M}{nN}} + \frac{\sum_{i \in I_k} \mu_i}{\mu_{i_k}^2} \sqrt{\frac{\mu_{i_k} p \log M}{nN}}.$$

Recall that  $\mu_i = \alpha_i \gamma_k / K$  for any  $i \in I_k$  in (15). We further have

$$\frac{1}{\mu_{i_k}} \sum_{i \in I_k} \sqrt{\frac{\mu_i p \log M}{nN}} + \frac{\sum_{i \in I_k} \mu_i}{\mu_{i_k}^2} \sqrt{\frac{\mu_{i_k} p \log M}{nN}} = \frac{1}{\alpha_{i_k}} \sqrt{\frac{pK \log M}{\gamma_k nN}} \left[ \sum_{i \in I_k} \sqrt{\alpha_i} + \frac{\sum_{i \in I_k} \alpha_i}{\sqrt{\alpha_{i_k}}} \right]$$

and we conclude that, on the event  $\mathcal{E}$ ,

$$\|\hat{B}_{Ik} - B_{Ik}\|_1 \lesssim \frac{\sum_{i \in I_k} \alpha_i}{\alpha_{i_k} \sqrt{\underline{\alpha}_I} \gamma_k} \sqrt{\frac{pK \log M}{nN}}. \quad (58)$$

We proceed to show step (2). Recall that  $\hat{\Omega} = (\hat{\omega}_1, \dots, \hat{\omega}_K)$  is the optimal solution from (41),  $\hat{B}_J = (\hat{\Theta}_{JL} \hat{\Omega})_+$  and  $B_J = \Theta_{JL} \Omega$ . Fix any  $1 \leq k \leq K$  and denote the canonical basis vectors in  $\mathbb{R}^K$  by  $e_1, \dots, e_K$ . Since  $B$  has only non-negative entries, we have

$$\begin{aligned} & \|\hat{B}_{Jk} - B_{Jk}\|_1 \\ &= \|(\hat{\Theta}_{JL} \hat{\Omega}_{\cdot k})_+ - \Theta_{JL} \Omega_{\cdot k}\|_1 \\ &\leq \|\hat{\Theta}_{JL} \hat{\Omega}_{\cdot k} - \Theta_{JL} \Omega_{\cdot k}\|_1 \\ &\leq \|(\hat{\Theta}_{JL} - \Theta_{JL}) \hat{\Omega}_{\cdot k}\|_1 + \|\Theta_{JL} \hat{\Omega}_{\cdot k} - B_{Jk}\|_1 \\ &\leq \|\hat{\Omega}_{\cdot k}\|_1 \|\hat{\Theta}_{JL} - \Theta_{JL}\|_{1,\infty} + \|B_J \Theta_{LL} \hat{\Omega}_{\cdot k} - B_J e_k\|_1 \\ &\leq \|\hat{\Omega}_{\cdot k}\|_1 \|\hat{\Theta}_{JL} - \Theta_{JL}\|_{1,\infty} + \left[ \|\hat{\Theta}_{LL} \hat{\Omega}_{\cdot k} - e_k\|_1 + \|(\hat{\Theta}_{LL} - \Theta_{LL}) \hat{\Omega}_{\cdot k}\|_1 \right] \|B_J\|_{1,\infty} \\ &\leq \|\hat{\omega}_k\|_1 \|\hat{\Theta}_{JL} - \Theta_{JL}\|_{1,\infty} + \left[ \|\hat{\Theta}_{LL} \hat{\Omega}_{\cdot k} - e_k\|_1 + \|\hat{\omega}_k\|_1 \|\hat{\Theta}_{LL} - \Theta_{LL}\|_{\infty,1} \right] \|B_J\|_{1,\infty}. \end{aligned}$$

We first study the property of  $\hat{\Omega}$ . Notice that  $\omega_k := \Omega_{\cdot k}$  is feasible of (41) since, on the event  $\mathcal{E}$ ,

$$\|\hat{\Theta}_{LL} \omega_k - e_k\|_1 \leq \|\omega_k\|_1 \|\hat{\Theta}_{LL} - \Theta_{LL}\|_{\infty,1} \stackrel{\mathcal{E}}{\leq} C_0 \|\omega_k\|_1 \max_{i \in L} \sum_{j \in L} \eta_{ij} = \|\omega_k\|_1 \lambda,$$

by Proposition 8. The optimality and feasibility of  $\hat{\omega}_k$  imply

$$\|\hat{\omega}_k\|_1 \leq \|\omega_k\|_1, \quad \|\hat{\Theta}_{LL} \hat{\omega}_k - e_k\|_1 \leq \|\hat{\omega}_k\|_1 \lambda \leq \|\omega_k\|_1 \lambda.$$

Hence, on the event  $\mathcal{E}$ , we have

$$\|\hat{B}_{Jk} - B_{Jk}\|_1 \leq C_0 \|\omega_k\|_1 \max_{i \in L} \sum_{j \in J} \eta_{ij} + 2 \|\omega_k\|_1 \lambda \|B_J\|_{1,\infty}.$$

Recall that  $B_J = A_J A_L^{-1}$  and  $A_L = \text{diag}(\alpha_{i_1}/p, \dots, \alpha_{i_K}/p)$ , and deduce

$$\|B_J\|_{1,\infty} = \max_{1 \leq k \leq K} \frac{p}{\alpha_{i_k}} \sum_{j \in J} A_{jk} \leq \frac{p}{\underline{\alpha}_I} \|A_J\|_{1,\infty} \quad (59)$$

Recall that  $\lambda = \max_{i \in L} \sum_{j \in L} \eta_{ij}$  and notice that

$$\|\omega_k\|_1 = \|\Omega_{\cdot k}\|_1 = \|\Theta_{LL}^{-1} e_k\|_1 = \|A_L^{-1} C^{-1} A_L^{-1} e_k\|_1 \leq \frac{p^2}{\alpha_{i_k} \underline{\alpha}_I} \|C^{-1}\|_{\infty,1}. \quad (60)$$

Collecting (59) – (60) gives

$$\|\widehat{B}_{Jk} - B_{Jk}\|_1 \leq C_0 \frac{p^2}{\alpha_{i_k} \underline{\alpha}_I} \|C^{-1}\|_{\infty,1} \left[ \max_{i \in L} \sum_{j \in J} \eta_{ij} + 2p \frac{\|A_J\|_{1,\infty}}{\underline{\alpha}_I} \max_{i \in L} \sum_{j \in L} \eta_{ij} \right].$$

Invoking (51) – (52) in Lemma 13 yields, on the event  $\mathcal{E}$ ,

$$\begin{aligned} \|\widehat{B}_{Jk} - B_{Jk}\|_1 &\lesssim \frac{p^2 \|C^{-1}\|_{\infty,1}}{\alpha_{i_k} \underline{\alpha}_I} \left[ \sqrt{\bar{\alpha}_I \gamma} S_J \sqrt{\frac{\log M}{K n p^2 N}} + \frac{\|A_J\|_{1,\infty}}{\underline{\alpha}_I} \sqrt{\bar{\alpha}_I^3 \gamma} \sqrt{\frac{\log M}{n p N}} \right] \\ &\leq \frac{p}{\alpha_{i_k}} \|C^{-1}\|_{\infty,1} \frac{\bar{\alpha}_I}{\underline{\alpha}_I} \sqrt{\frac{\gamma \log M}{K n N}} \left[ \sqrt{|J| + \sum_{j \in J} \frac{\alpha_j}{\bar{\alpha}}} + \frac{\bar{\alpha}_I}{\underline{\alpha}_I} \sqrt{K \sum_{j \in J} \frac{\alpha_j}{\bar{\alpha}_I}} \right] \end{aligned} \quad (61)$$

where we recall that  $S_J = |J| \bar{\alpha}_I + \sum_{j \in J} \alpha_j$  and use  $\|A_J\|_{1,\infty} \leq 1$ ,  $\|A_J\|_{1,\infty} \leq \sum_{j \in J} \alpha_j / p$  in the second inequality. Combining (58) and (61) yields, on the event  $\mathcal{E}$ ,

$$\begin{aligned} \|\widehat{B}_{\cdot k} - B_{\cdot k}\|_1 &\lesssim \frac{p}{\alpha_{i_k}} \frac{\sum_{i \in I_k} \alpha_i}{\sqrt{\bar{\alpha}_I \gamma_k}} \sqrt{\frac{K \log M}{n p N}} \\ &\quad + \frac{p}{\alpha_{i_k}} \|C^{-1}\|_{\infty,1} \frac{\bar{\alpha}_I}{\underline{\alpha}_I} \sqrt{\frac{\gamma \log M}{K n N}} \left[ \sqrt{|J| + \sum_{j \in J} \frac{\alpha_j}{\bar{\alpha}}} + \frac{\bar{\alpha}_I}{\underline{\alpha}_I} \sqrt{K \sum_{j \in J} \frac{\alpha_j}{\bar{\alpha}_I}} \right]. \end{aligned} \quad (62)$$

It remains to prove step (3). For any  $k \in [K]$ , from (44), we have

$$\begin{aligned} |\widehat{A}_{jk} - A_{jk}| &= \left| \frac{\widehat{B}_{jk}}{\|\widehat{B}_{\cdot k}\|_1} - \frac{B_{jk}}{\|B_{\cdot k}\|_1} \right| \\ &\leq \frac{\widehat{B}_{jk}}{\|\widehat{B}_{\cdot k}\|_1 \|B_{\cdot k}\|_1} \left| \|\widehat{B}_{\cdot k}\|_1 - \|B_{\cdot k}\|_1 \right| + \frac{|\widehat{B}_{jk} - B_{jk}|}{\|B_{\cdot k}\|_1} \\ &= \frac{\left| \|\widehat{B}_{\cdot k}\|_1 - \|B_{\cdot k}\|_1 \right|}{\|B_{\cdot k}\|_1} \widehat{A}_{jk} + \frac{|\widehat{B}_{jk} - B_{jk}|}{\|B_{\cdot k}\|_1} \end{aligned}$$

by using  $\widehat{A}_{jk} = \widehat{B}_{jk} / \|\widehat{B}_{\cdot k}\|_1$  in the last equality. Since  $\|\widehat{A}_{\cdot k}\|_1 = 1$ , summing over  $j \in [p]$  yields

$$\|\widehat{A}_{\cdot k} - A_{\cdot k}\|_1 \leq \frac{2 \|\widehat{B}_{\cdot k} - B_{\cdot k}\|_1}{\|B_{\cdot k}\|_1} = \frac{2 \alpha_{i_k}}{p} \|\widehat{B}_{\cdot k} - B_{\cdot k}\|_1.$$

The equality uses  $\|B_{\cdot k}\|_1 = p / \alpha_{i_k}$  from  $B = A A_L^{-1}$ . Invoking (62) concludes the proof.  $\square$

## D.2.2. Proof of Corollary 8

To prove Corollary 8, we need the following lemma which controls  $\|C^{-1}\|_{\infty,1}$ .

**Lemma 14.** *Let  $\bar{\gamma}$  and  $\underline{\gamma}$  be defined in (45). Assume  $\bar{\gamma} \asymp \underline{\gamma}$  and  $\sum_{k' \neq k} \sqrt{C_{kk'}} = o(\sqrt{C_{kk}})$  for any  $1 \leq k \leq K$ . Then  $\|C^{-1}\|_{\infty,1} = O(K)$ .*

**Proof.** From the definition of  $(\infty, 1)$ -norm and the symmetry of  $C$ , one has

$$\|C^{-1}\|_{\infty,1} = \sup_{v \neq 0} \frac{\|C^{-1}v\|_1}{\|v\|_1} = \sup_{v \neq 0} \frac{\|v\|_1}{\|Cv\|_1} = \left( \inf_{\|v\|_1=1} \|Cv\|_1 \right)^{-1}.$$

It suffices to lower bound  $\inf_{\|v\|_1=1} \|Cv\|_1$ . We have

$$\begin{aligned} \inf_{\|v\|_1=1} \|Cv\|_1 &= \inf_{\|v\|_1=1} \sum_{a=1}^K \left| C_{aa}v_a + \sum_{b \neq a} C_{ab}v_b \right| \\ &\geq \inf_{\|v\|_1=1} \sum_{a=1}^K \left( C_{aa}|v_a| - \sum_{b \neq a} C_{ab}|v_b| \right) \\ &= \inf_{\|v\|_1=1} \sum_{a=1}^K C_{aa}|v_a| - \sum_{b=1}^K |v_b| \sum_{a \neq b} C_{ab}. \end{aligned}$$

Note that  $\sum_{k' \neq k} \sqrt{C_{kk'}} = o(\sqrt{C_{kk}})$  implies

$$\sum_{k' \neq k} C_{kk'} \leq \left( \sum_{k' \neq k} \sqrt{C_{kk'}} \right)^2 = o(C_{kk}), \quad \text{for any } k \in [K] \quad (63)$$

and  $C_{kk} \leq n^{-1} \|W_k\|_1 = \gamma_k/K = O(1/K)$  by using  $\bar{\gamma} \asymp \underline{\gamma} \asymp 1$ . We further obtain

$$\inf_{\|v\|_1=1} \|Cv\|_1 \gtrsim \inf_{\|v\|_1=1} \sum_{a=1}^K (C_{aa}|v_a| - |v_b|o(1/K)) \gtrsim \min_a C_{aa}.$$

Observe that

$$\frac{1}{K} - C_{kk} \asymp \frac{\gamma_k}{K} - C_{kk} = \sum_{k'=1}^K C_{kk'} - C_{kk} = \sum_{k' \neq k} C_{kk'} \leq \sum_{k' \neq k} \sqrt{C_{kk'}} = o(C_{kk}).$$

This implies  $C_{kk} \asymp 1/K$  which concludes  $\inf_{\|v\|_1=1} \|Cv\|_1 \gtrsim 1/K$  and completes the proof.  $\square$

**Proof of Corollary 8.** From (53) in Lemma 13, under  $\sum_{k' \neq k} \sqrt{C_{kk'}} = o(\sqrt{C_{kk}})$  for any  $1 \leq k \leq K$ , one has

$$\max_{i \in L} \sum_{j \in L} \eta_{ij} \lesssim \sqrt{\frac{\bar{\alpha}_I^3 \bar{\gamma} \log M}{K n p^3 N}}$$

which improves the rate in (51) by a factor of  $\sqrt{1/K}$ . Repeating the previous arguments for proving Theorem 7, one can show that

$$\text{Rem}(J, k) \lesssim \sqrt{\frac{K \log M}{nN}} \cdot \frac{\bar{\gamma}^{1/2} \|C^{-1}\|_{\infty,1}}{K} \cdot \frac{\bar{\alpha}_I}{\underline{\alpha}_I} \left( \sqrt{|J| + \sum_{j \in J} \rho_j} + \frac{\bar{\alpha}_I}{\underline{\alpha}_I} \sqrt{\sum_{j \in J} \rho_j} \right).$$

Invoking conditions (i) – (ii) of Corollary 8 together with  $\|C^{-1}\|_{\infty,1} = O(K)$  from Lemma 14, one can obtain

$$\sum_{k=1}^K \text{Rem}(I, k) \lesssim \sum_{i \in I} \sqrt{\frac{\alpha_i K \log M}{n p N}} \leq K \sqrt{\frac{|I| \log M}{nN}}$$

by using Cauchy-Schwarz inequality with  $\sum_{i \in I} \alpha_i \leq \sum_{i=1}^p \alpha_i \leq pK$ , and

$$\text{Rem}(J, k) \lesssim \sqrt{\frac{|J| K \log M}{nN}}.$$

This yields the optimal rate of  $L_1(A, \hat{A})$ . For  $L_{1,\infty}(A, \hat{A})$ , observe that  $\sum_{i \in I_k} \alpha_i/p = \sum_{i \in I_k} A_{ik} \leq 1$ . This yields

$$\text{Rem}(I, k) \lesssim \sum_{i \in I_k} \sqrt{\frac{\alpha_i K \log M}{n p N}} \leq \sqrt{\frac{|I_k| K \log M}{nN}},$$

which, in conjunction with the rate of  $\text{Rem}(J, k)$ , concludes the result of  $L_{1,\infty}(A, \hat{A})$ .  $\square$

#### D.2.3. Proof of the statment in Remark 9

We prove the result of Theorem 7 when condition (26) is replaced by (27) and (49). First note that, similar as (13) and (26), condition (49) implies

$$\min_{j \in I} \frac{\mu_j}{p} = \min_{j \in I} \frac{1}{n} \sum_{i=1}^n \Pi_{ji} \geq \frac{c \log M}{N}, \quad \min_{j \in I} \frac{m_j}{p} = \min_{j \in I} \max_{1 \leq i \leq n} \Pi_{ji} \geq \frac{c' (\log M)^2}{N}. \quad (64)$$

We will work on the event  $\mathcal{E}'$  defined in the proof of Corollary 10 which holds with probability greater than  $1 - O(M^{-1})$  under condition (27). To prove Theorem 7, observe that its proof in Section D.2.1 only uses the result of Lemma 5, Lemma 13 and (29). Since Lemma 5 and (29) is guaranteed by  $\mathcal{E}'$ , it suffices to prove that Lemma 13 holds

for  $\eta_{j\ell}$  defined in (31). This is indeed true since the only different terms in the expression of  $\eta_{j\ell}$  in (31) than (50) are

$$\frac{m_j + m_\ell}{p} \vee \frac{\log^2 M}{N}, \quad \frac{\mu_j + \mu_\ell}{p} \vee \frac{\log M}{N}$$

for any  $j \in I_k$  and  $\ell \in [p]$ , and hence invoking (64) yields

$$\frac{m_j + m_\ell}{p} \vee \frac{\log^2 M}{N} \lesssim \frac{m_j + m_\ell}{p}, \quad \frac{\mu_j + \mu_\ell}{p} \vee \frac{\log M}{N} \lesssim \frac{\mu_j + \mu_\ell}{p}.$$

Therefore, Lemma 13 follows and so does Theorem 7.  $\square$

## Appendix E: Discussions of Assumptions 2 and 3

### E.1. Examples

The following example shows that Assumption 2 does not imply Assumption 3.

**Example 1.** In the first two instances (65) and (66) below, Assumptions 2 and 3 both hold. These instances give insight into why Assumption 3 may fail, while Assumption 2 holds, which is shown in the third instance (67).

We consider the following matrix

$$W = \begin{bmatrix} 0.5 & 0.4 & 0 & 0 & \mathbf{0.4} \\ 0.2 & 0.6 & 0.5 & 0.5 & \mathbf{0} \\ 0.3 & 0 & 0.5 & 0.5 & \mathbf{0.1} \\ \mathbf{0} & \mathbf{0} & \mathbf{0} & \mathbf{0} & \mathbf{0.5} \end{bmatrix} \implies \tilde{C} = \begin{bmatrix} 0.34 & 0.15 & 0.1 & 0.31 \\ 0.15 & 0.28 & 0.22 & 0 \\ 0.1 & 0.22 & 0.31 & 0.07 \\ 0.31 & 0 & 0.07 & 1 \end{bmatrix}. \quad (65)$$

Clearly, each diagonal entry of  $\tilde{C}$  dominates the non-diagonal ones, row-wise. From (23), Assumption 3 holds. Assumption 2 can be verified as well. We see that topic 4 is *rare*, in that it only occurs in document 5. However, the probability that the rare topic occurs is not small ( $W_{45} = 0.5$ ). Since each column sums to 1, the closer  $W_{45}$  is to 1, the smaller the other entries in the 5th column must be, and the more uncorrelated topic 4 will be with other topics. Hence, the larger  $W_{45}$ , the more likely it is that Assumption 3 holds. Suppose the rare topic 4 also has a small probability, for instance

$$W = \begin{bmatrix} 0.5 & 0.4 & 0 & 0 & \mathbf{0.3} \\ 0.2 & 0.6 & 0.5 & 0.5 & \mathbf{0.2} \\ 0.3 & 0 & 0.5 & 0.5 & \mathbf{0.4} \\ \mathbf{0} & \mathbf{0} & \mathbf{0} & \mathbf{0} & \mathbf{0.1} \end{bmatrix} \implies \tilde{C} = \begin{bmatrix} 0.35 & 0.17 & 0.13 & 0.25 \\ 0.17 & 0.24 & 0.19 & 0.1 \\ 0.13 & 0.19 & 0.26 & 0.24 \\ 0.25 & 0.1 & 0.24 & 1 \end{bmatrix}. \quad (66)$$

While the rare topic 4 has small non-zero entry  $W_{45} = 0.1$ , none of  $W_{i5}$  for  $i = 1, 2, 3$ , is dominating and Assumption 3 is still met. However, it fails in the following scenario:

$$W = \begin{bmatrix} 0.5 & 0.4 & 0 & 0 & \mathbf{0.9} \\ 0.2 & 0.6 & 0.5 & 0.5 & \mathbf{0} \\ 0.3 & 0 & 0.5 & 0.5 & \mathbf{0} \\ \mathbf{0} & \mathbf{0} & \mathbf{0} & \mathbf{0} & \mathbf{0.1} \end{bmatrix} \implies \tilde{C} = \begin{bmatrix} \mathbf{0.38} & 0.1 & 0.06 & \mathbf{0.5} \\ 0.1 & 0.28 & 0.24 & 0 \\ 0.06 & 0.24 & 0.35 & 0 \\ \mathbf{0.5} & 0 & 0 & 1 \end{bmatrix}. \quad (67)$$

Here, a frequent topic (topic 1) has probability  $W_{15} = 0.9$ , that dominates all other entries in the fifth column. Topic 4 is hard to detect since it occurs with probability 0.1, while the frequent topic 1 occurs with probability 0.9, in the single document that may reveal topic 4. We emphasize that  $W$  in all three cases above satisfy Assumption 2.

We give an example below to show that Assumption 3 does not imply Assumption 2, that is,  $W$  satisfies Assumption 3 but does not have rank  $K$ .

**Example 3** Let  $K = n = 5$  and consider

$$W = \begin{bmatrix} 0.3 & 0.05 & 0.3 & 0 & 0 \\ 0.25 & 0.04 & 0.25 & 0.32 & 0.1 \\ 0 & 0.5 & 0.15 & 0.1 & 0.3 \\ 0.055 & 0.257 & 0.13 & 0.466 & 0.28 \\ 0.395 & 0.153 & 0.17 & 0.114 & 0.32 \end{bmatrix}.$$

Note that  $W_{4\cdot} = -0.9W_{1\cdot} + 1.3W_{2\cdot} + 0.5W_{3\cdot}$ , which implies  $\text{rank}(W) < 5$ . However, it follows that

$$\tilde{C} = n\tilde{W}\tilde{W}^T = \begin{bmatrix} \mathbf{2.16} & 1.22 & 0.51 & 0.44 & 1.18 \\ 1.22 & \mathbf{1.3} & 0.59 & 1.02 & 0.98 \\ 0.51 & 0.59 & \mathbf{1.69} & 1.12 & 0.87 \\ 0.44 & 1.02 & 1.12 & \mathbf{1.35} & 0.83 \\ 1.18 & 0.98 & 0.87 & 0.83 & \mathbf{1.22} \end{bmatrix}.$$

Therefore, Assumption 3 is satisfied as it is equivalent with  $\tilde{C}_{ii} \wedge \tilde{C}_{jj} > \tilde{C}_{ij}$  for any  $i, j \in [K]$ , whereas  $W$  does not have full rank.

## E.2. Statements and proofs of results invoked in Remark 3

We first show the equivalence between  $\nu > 4\delta$  and

$$\cos(\angle(W_{i\cdot}, W_{j\cdot})) < \left( \frac{\zeta_i}{\zeta_j} \wedge \frac{\zeta_j}{\zeta_i} \right) \left( 1 - \frac{4\delta}{n\zeta_i\zeta_j} \right), \quad \text{for all } 1 \leq i \neq j \leq K. \quad (68)$$

**Lemma 15.** *Let  $\nu$  be defined in (23) with  $\tilde{C} = n\tilde{W}\tilde{W}^T$  and  $\tilde{W} = D_W^{-1}W$ . Then, the inequality  $\nu > 4\delta$  is equivalent with (68). In particular,  $\nu > 0$  is equivalent with Assumption 3.*

**Proof.** Starting with the definition of  $\nu$ , we have

$$\begin{aligned} \nu &> 4\delta \\ \iff \frac{n\|W_{i\cdot}\|_2^2}{\|W_{i\cdot}\|_1^2} \wedge \frac{n\|W_{j\cdot}\|_2^2}{\|W_{j\cdot}\|_1^2} - \frac{n\langle W_{i\cdot}, W_{j\cdot} \rangle}{\|W_{i\cdot}\|_1\|W_{j\cdot}\|_1} &> 4\delta, \quad \text{for all } i \neq j \\ \iff n\zeta_i^2 \wedge n\zeta_j^2 - n\zeta_i\zeta_j \cos(\angle(W_{i\cdot}, W_{j\cdot})) &> 4\delta, \quad \text{for all } i \neq j \end{aligned}$$

by using  $\zeta_i = \|W_{i\cdot}\|_2/\|W_{i\cdot}\|_1$ . The result follows after rearranging terms, and taking  $\delta = 0$  we obtain the second assertion as well.  $\square$

The following lemma provides an upper bound of  $\delta$  defined in (24).

**Lemma 16.** *Assume condition (26) holds. Then, there exists some constant  $c > 0$  such that*

$$\delta \leq c \left\{ \max_{\ell \in [p]} \frac{m_\ell}{\mu_\ell} \sqrt{\frac{1}{n}} + \sqrt{\frac{\log M}{n}} \right\} := \varepsilon_n.$$

If, in addition,  $\log M = o(n)$  and condition (33) hold, we have

$$\frac{\delta}{n \min_i \zeta_i^2} = o(1)$$

with  $\zeta_i = \|W_{i\cdot}\|_2/\|W_{i\cdot}\|_1$ .

**Proof.** First, we notice that  $\delta = \max_{1 \leq j \leq p} \delta_{jj}$ . For any  $1 \leq j \leq p$ , the expressions in (17) – (18) yield

$$\delta_{jj} \asymp \frac{p^2}{\mu_j^2} \left\{ \sqrt{\frac{m_j \Theta_{jj} \log M}{npN}} + \frac{m_j \log M}{npN} + \sqrt{\frac{\mu_j (\log M)^4}{npN^3}} + \Theta_{jj} \sqrt{\frac{p \log M}{\mu_j nN}} \right\}.$$

Using

$$\Theta_{jj} = \frac{1}{n} \sum_{i=1}^n \Pi_{ji}^2 \leq \frac{1}{n} \sum_{i=1}^n \Pi_{ji} \max_{1 \leq i \leq n} \Pi_{ji} \stackrel{(2)}{=} \frac{\mu_j m_j}{p^2}, \quad (69)$$

together with (13), we obtain

$$\begin{aligned} \delta_{jj} &\lesssim \frac{m_j}{\mu_j} \sqrt{\frac{p \log M}{\mu_j nN}} + \frac{m_j p \log M}{\mu_j^2 nN} + \sqrt{\frac{p^3 (\log M)^4}{\mu_j^3 nN^3}} \\ &\lesssim \frac{m_j}{\mu_j} \sqrt{\frac{1}{n}} + \sqrt{\frac{\log M}{n}} \end{aligned} \quad (70)$$

Taking the maximum over  $j \in [p]$  concludes the proof of the upper bound of  $\delta$ . The second part follows by observing that

$$\min_{1 \leq i \leq K} n \zeta_i^2 = \min_{1 \leq i \leq K} \frac{n \|W_{i\cdot}\|_2^2}{\|W_{i\cdot}\|_1^2} \geq 1,$$

by the Cauchy-Schwarz inequality.  $\square$

### E.3. The Dirichlet distribution of $W$

Suppose the columns of  $W = (W_1, \dots, W_n)$  are i.i.d. samples from the Dirichlet distribution parametrized by the vector  $d = (d_1, \dots, d_K) \in \mathbb{R}^K$ . Let  $d_0 := \sum_k d_k$ . It is well known that, for any  $1 \leq k \leq K$ ,

$$a_k := \mathbb{E}[W_{ki}] = \frac{d_k}{d_0}, \quad \sigma_{kk}^2 := \text{Var}(W_{ki}) = \frac{d_k(d_0 - d_k)}{d_0^2(d_0 + 1)} \quad (71)$$

and, for any  $1 \leq k \neq \ell \leq K$ ,

$$s_{kk} := \mathbb{E}[W_{ki}^2] = \frac{d_k(1 + d_k)}{d_0(1 + d_0)}, \quad s_{k\ell} := \mathbb{E}[W_{ki}W_{\ell i}] = \frac{d_k d_\ell}{d_0(1 + d_0)}. \quad (72)$$

Further denote

$$\hat{a}_k := \frac{1}{n} \sum_{i=1}^n W_{ki}, \quad \hat{s}_{k\ell} = \frac{1}{n} \sum_{i=1}^n W_{ki}W_{\ell i}, \quad \text{for any } 1 \leq k, \ell \leq K$$

and the event

$$\mathcal{E}_{dir} = \{|\hat{a}_k - a_k| \leq \varepsilon_1^k, \quad |\hat{s}_{k\ell} - s_{k\ell}| \leq \varepsilon_2^{k\ell}, \quad \text{for all } 1 \leq k, \ell \leq K\}. \quad (73)$$

From Lemma 15, condition  $\nu > 4\delta$  discussed in Remark 3 is equivalent with

$$\frac{\hat{s}_{kk}}{\hat{a}_k^2} \wedge \frac{\hat{s}_{\ell\ell}}{\hat{a}_\ell^2} - \frac{\hat{s}_{k\ell}}{\hat{a}_k \hat{a}_\ell} > 4\delta, \quad \text{for any } 1 \leq k < \ell \leq K. \quad (74)$$

In particular, Assumption 3 corresponds to  $\delta = 0$  in (74). The following lemma provides sufficient conditions that guarantee Assumption 3 and  $\nu > 4\delta$ . Recall that  $M := n \vee p \vee \max_{i \in [n]} N_i$ .

**Lemma 17.** *Assume the columns of  $W$  are i.i.d. from a Dirichlet distribution with parameter  $d = (d_1, \dots, d_K)$ . Set  $d_0 := d_1 + \dots + d_K$ ,  $\bar{d} := \max_k d_k$  and  $\underline{d} := \min_k d_k$ . Assumption 3 holds with probability greater than  $1 - O(M^{-1})$ , provided*

$$\frac{1 \vee \bar{d}}{\underline{d}} d_0(1 + d_0) \leq c \frac{n}{\log M} \quad (75)$$

*holds, for some constant  $c > 0$  sufficiently small. Additionally, if*

$$\frac{\bar{d}(1 + d_0)}{\underline{d}} \leq c \sqrt{\frac{n}{\log M}}, \quad (76)$$

*holds for some constant  $c > 0$  small enough, then  $\mathbb{P}\{\nu > 4\delta\} \geq 1 - O(M^{-1})$ .*

**Proof.** Display (70) together with

$$\frac{m_j}{p} = \max_{1 \leq t \leq n} \Pi_{jt} \leq \|A_{j\cdot}\|_1, \quad \frac{\mu_j}{p} = \frac{1}{n} \sum_{t=1}^n \Pi_{jt} \geq \|A_{j\cdot}\|_1 \min_k \frac{1}{n} \|W_{k\cdot}\|_1 = \|A_{j\cdot}\|_1 \min_k \hat{a}_k$$

from (14) and (16) yield

$$\delta \lesssim \frac{1}{\min_k \hat{a}_k} \sqrt{\frac{1}{n}} + \sqrt{\frac{\log M}{n}}. \quad (77)$$

We work on the event  $\mathcal{E}_{dir}$  with  $\varepsilon_1^k$  and  $\varepsilon_2^{k\ell}$  chosen as

$$\varepsilon_1^k = c_1 \sqrt{\frac{d_k}{d_0(1+d_0)}} \sqrt{\frac{\log M}{n}}, \quad \varepsilon_2^{k\ell} = c_2 \left\{ \sqrt{\frac{d_k d_\ell}{d_0(1+d_0)}} + \sqrt{\frac{\log M}{n}} \right\} \sqrt{\frac{\log M}{n}}, \quad (78)$$

for any  $1 \leq k \leq \ell \leq K$  where  $c_1, c_2$  are some positive constants such that, from Lemma 18,  $\mathbb{P}(\mathcal{E}_{dir}) \geq 1 - O(M^{-1})$ . Note that condition (75) and  $\mathcal{E}_{dir}$  imply

$$\hat{a}_k \leq a_k + \varepsilon_1^k \leq \frac{d_k}{d_0} + c_1 \sqrt{\frac{d_k}{d_0(1+d_0)}} \sqrt{\frac{\log M}{n}} \leq c'_1 a_k; \quad (79)$$

$$\hat{a}_k \geq a_k - \varepsilon_1^k \leq \frac{d_k}{d_0} - c_1 \sqrt{\frac{d_k}{d_0(1+d_0)}} \sqrt{\frac{\log M}{n}} \geq c''_1 a_k \quad (80)$$

for all  $k \in [K]$ . In the following, we prove (74) by only showing

$$\frac{\hat{s}_{kk}}{\hat{a}_k^2} - \frac{\hat{s}_{k\ell}}{\hat{a}_k \hat{a}_\ell} = \frac{\hat{s}_{kk} \hat{a}_\ell - \hat{s}_{k\ell} \hat{a}_k}{\hat{a}_k^2 \hat{a}_\ell} > 4\delta \quad (81)$$

since the other part can be deduced by using similar arguments. We first show that, on the event  $\mathcal{E}_{dir}$ , condition (75) guarantees

$$\frac{\hat{s}_{kk} \hat{a}_\ell - \hat{s}_{k\ell} \hat{a}_k}{\hat{a}_k^2 \hat{a}_\ell} \geq \rho \cdot \frac{d_0}{d_k(1+d_0)}$$

for some constant  $\rho \in [0, 1)$ . We bound the numerator of the term on the left from below by

$$\begin{aligned} \hat{s}_{kk} \hat{a}_\ell - \hat{s}_{k\ell} \hat{a}_k &\geq (s_{kk} - \varepsilon_2^{kk}) (a_\ell - \varepsilon_1^\ell) - (s_{k\ell} + \varepsilon_2^{k\ell}) (a_k + \varepsilon_1^k) \\ &= s_{kk} a_\ell - s_{k\ell} a_k - \varepsilon_2^{kk} c'_1 a_\ell - \varepsilon_1^\ell s_{kk} - \varepsilon_2^{k\ell} c'_1 a_k - \varepsilon_1^k s_{k\ell} \\ &= \frac{d_k d_\ell}{d_0^2(1+d_0)} - c'_1 \varepsilon_2^{kk} \frac{d_\ell}{d_0} - \varepsilon_1^\ell \frac{d_k(1+d_k)}{d_0(1+d_0)} - c'_1 \varepsilon_2^{k\ell} \frac{d_k}{d_0} - \varepsilon_1^k \frac{d_k d_\ell}{d_0(1+d_0)}. \end{aligned}$$

We used (79) in the second line and used (71) – (72) in the third line. We then show that

$$\max \left\{ c'_1 \varepsilon_2^{kk} \frac{d_\ell}{d_0}, \varepsilon_1^\ell \frac{d_k(1+d_k)}{d_0(1+d_0)}, c'_1 \varepsilon_2^{k\ell} \frac{d_k}{d_0}, \varepsilon_1^k \frac{d_k d_\ell}{d_0(1+d_0)} \right\} \leq \frac{d_k d_\ell}{5d_0^2(1+d_0)}.$$

From (71) – (72), it suffices to show the individual inequalities

$$5c'_1\varepsilon_2^{kk} < \frac{d_k}{d_0(1+d_0)}, \quad 5\varepsilon_1^\ell < \frac{d_\ell}{d_0(1+d_k)}, \quad 5c'_1\varepsilon_2^{k\ell} < \frac{d_\ell}{d_0(1+d_0)}, \quad 5\varepsilon_1^k < \frac{1}{d_0}.$$

These inequalities follow by invoking condition (75) and plugging in the expression of  $\varepsilon_1^k$  and  $\varepsilon_2^{k\ell}$  in (78). We thus have

$$\widehat{s}_{kk}\widehat{a}_\ell - \widehat{s}_{k\ell}\widehat{a}_k \geq \frac{1}{5} \frac{d_k d_\ell}{d_0^2(1+d_0)}.$$

In conjunction with (79), we conclude that

$$\frac{\widehat{s}_{kk}\widehat{a}_\ell - \widehat{s}_{k\ell}\widehat{a}_k}{\widehat{a}_k^2\widehat{a}_\ell} \geq \frac{1}{5(c'_1)^3} \frac{d_0}{d_k(1+d_0)}$$

which further yields

$$\frac{\widehat{s}_{kk}}{\widehat{a}_k^2} \wedge \frac{\widehat{s}_{\ell\ell}}{\widehat{a}_\ell^2} - \frac{\widehat{s}_{k\ell}}{\widehat{a}_k\widehat{a}_\ell} \geq \frac{1}{5(c'_1)^3} \frac{d_0}{\bar{d}(1+d_0)}.$$

When  $\delta = 0$ , the first statement follows. To prove the statement of  $\nu > 4\delta$ , it suffices to show

$$\frac{1}{5(c'_1)^3} \frac{d_0}{\bar{d}(1+d_0)} > 4\delta.$$

This follows by invoking (76), (77) and (80). The proof is complete.  $\square$

**Remark 4.** For a symmetric Dirichlet distribution, that is,  $d_1 = \dots = d_K = d$ , condition (76) and (75) becomes, respectively,

$$1 + Kd \leq c\sqrt{\frac{n}{\log M}}, \quad (1 \vee d)K(1 + Kd) \leq c\frac{n}{\log M}.$$

The larger  $K$  is, the smaller  $d/n$  needs to be. Note that small  $d$  encourages the sparsity of  $W$ .

**Lemma 18.** Under condition (75), assume columns of  $W$  are i.i.d. sample from the Dirichlet distribution. Then  $\mathbb{P}(\mathcal{E}_{dir}) \geq 1 - M^{-1}$  with  $\varepsilon_1^k$  and  $\varepsilon_2^{k\ell}$  chosen as (78).

**Sketch of the proof.** Since  $W_{ki}$  and  $W_{ki}W_{\ell i}$  are bounded by 1 and displays (71) – (72) imply  $\text{Var}(W_{ki}W_{\ell i}) \leq d_k d_\ell / (d_0(1+d_0))$ , using Bernstein's inequality in Lemma 3 with similar arguments in Lemmas 5 and 7 together with condition (75) yield the desired result.  $\square$

## Appendix F: Cross-validation procedure for selecting $C_1$ in Algorithm 3

We give a practical cross-validation procedure for selecting the proportionally constant  $C_1$  used in Algorithm 3. Starting with a chosen fine grid  $\mathcal{C}$ , we randomly split the data into a training set  $\mathcal{D}_1$  and a validation set  $\mathcal{D}_2$ . For each  $c \in \mathcal{C}$ , we apply Algorithm 3 with  $T = 1$ ,  $C_0 = 0.01$  and  $C_1 = c$  on  $\mathcal{D}_1$  to obtain  $\hat{A}_c$  and  $\hat{C}_c$ , and then calculate the out-of-sample error

$$L(c) := \left\| \hat{\Theta}^{(2)} - \hat{A}_c \hat{C}_c \hat{A}_c^T \right\|_1.$$

Here  $\hat{\Theta}^{(2)}$  is obtained as in (20) by using  $\mathcal{D}_2$  and  $\|\cdot\|_1$  denotes the matrix  $\ell_1$  norm. The selected  $\hat{C}_1$  is defined as

$$\hat{C}_1 = \arg \min_{c \in \mathcal{C}} L(c).$$

Using estimates  $\hat{I}$  and  $\hat{A}$  and motivated by the structure  $\Theta_{II} = A_I C A_I^T$ , we can estimate  $C$  by

$$\hat{C} = (\hat{A}_I^T \hat{A}_I)^{-1} \hat{A}_I^T \hat{\Theta}_{II} \hat{A}_I (\hat{A}_I^T \hat{A}_I)^{-1}.$$

## Appendix G: Additional simulation results

### Sensitivity to topics number $K$

We study the performance of RECOVER-L2 and RECOVER-KL for different  $K$ . We show that even in a favorable low dimensional setting ( $p = 400$  and true  $K_0 = 15$ ) with  $|I_k| = 1$ ,  $\xi = 1/p$  and large sample sizes ( $N = 800$ ,  $n = 1000$ ), the estimation error is seriously affected by a wrong choice of the number of topics  $K$ .

We generated 50 datasets according to our data generating mechanism and applied RECOVER-L2, RECOVER-KL by using different  $K$  to each dataset to obtain  $\hat{A}_K$ . To quantify the estimation error, we use the criterion

$$\left\| \hat{A}_K \hat{A}_K^T - A A^T \right\|_1$$

to evaluate the overall fit of the word by word membership matrix  $A A^T \in \mathbb{R}^{p \times p}$ . We averaged this loss over 50 datasets. To further benchmark the result, we use a random guessing method UNIFORM which randomly draws  $p \times K$  entries from the Uniform(0, 1) distribution and normalizes each column to obtain an “estimate” that is independent of the data. The performance of RECOVER-L2, RECOVER-KL and UNIFORM is shown in Figure 1. It clearly shows that both RECOVER-L2 and RECOVER-KL are very sensitive indeed to correctly specified  $K$ . When  $K$  differs from the true value  $K_0$  by more than 2 units, the performance is close to random guessing! This phenomenon continues to hold for various settings and we conclude that specifying  $K$  is critical for both RECOVER-L2 and RECOVER-KL.

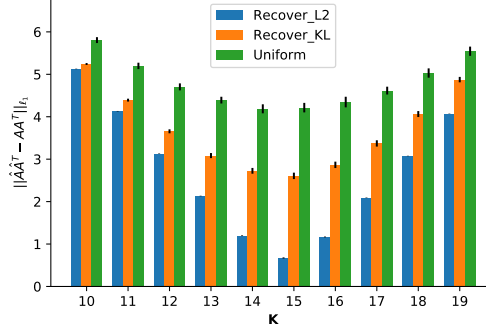

Figure 1: Plot of  $\|\hat{A}\hat{A}^T - AA^T\|_1$  for using different specified  $K$ . The black vertical bars are standard errors over 50 datasets.

## Comparison of different algorithms for small $K$

We compare TOP10, RECOVER-L2, RECOVER-KL and T-SCORE in the benchmark setting  $N = n = 1500$ ,  $p = 1000$  and  $\xi = 1/p$ , but for small values of  $K$ . T-SCORE is the procedure of [3], who kindly made the code available to us. Since  $K$  is small, the cardinality of each column  $W_i$  of  $W$  is randomly sampled from  $\{1, 2, 3\}$ .

In the first experiment, we considered  $K = 5$  and varied  $|I_k|$  within  $\{2, 3, 4, 5, 6\}$ . The estimation error  $L_1(\hat{A}, A)/K$ , averaged over 50 generated datasets, is shown in Figure 2. We see that the performance of RECOVER-KL is as good as TOP10 and even better for  $|I_k| \leq 3$ . However, as already verified in Section 6, RECOVER-KL has the worst performance for large  $K$  and is computationally demanding. The plot also demonstrates that T-SCORE needs at least 4 anchor words per group in order to have comparable performance with TOP10 and RECOVER-KL. This is as expected since  $|I_k|$  needs to grow as  $p^2 \log^2(n)/(nN)$  in [3].

In the second experiment, we set  $|I_k| = p/100$  and varied  $K$  from  $\{5, 6, \dots, 10\}$ . We considered this range of values as, unfortunately, in the implementation of T-SCORE the authors made available to us, it often crashes for  $K = 11$ . The average overall  $L_1$  estimation error in Figure 2 shows that TOP10 has the smallest error over all  $K$ . T-SCORE has similar performance when  $K \leq 8$  but becomes worse than TOP10 when  $K$  becomes larger.

## The New York Times (NYT) dataset

Similar to the procedure for preprocessing the NIPs dataset, we removed common stopping words and rare words occurring in less than 150 documents. The dataset after preprocessing has  $n = 299419$ ,  $p = 3079$  and  $N = 210$ . Since [1] mainly considers  $K = 100$ , we tune our method to obtain a similar number of topics for our comparative study, for both the semi-synthetic data and the real data.

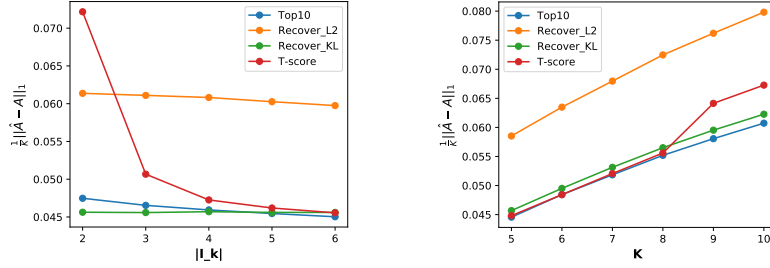

Figure 2: The left plot is the averaged *overall estimation error* by varying  $|I_k|$  and setting  $K = 5$ . The right one is for varying  $K$  and setting  $|I_k| = p/100$ .

**Semi-synthetic data comparison.** To generate the semi-synthetic data, we first apply TOP1 to the preprocessed dataset with  $C_0 = 0.01$  and  $C_1 = 15.5$ <sup>1</sup> and obtain the estimated word-to-topic matrix  $\hat{A}$  with  $\hat{K} = 101$  and 206 anchor words. Using this  $\hat{A}$ , we generate  $W$  from the previous three distributions (a) – (c), separately, with  $n = \{40000, 50000, 60000, 70000\}$ , and then generate  $X$  based on  $\hat{A}W$  with  $N = 250$ . For each setting, we generate 15 datasets and the averaged *overall estimation error* and *topic-wise estimation error* of TOP, RECOVER-L2, RECOVER-KL and LDA are reported in Figure 3. The running time of different algorithm is shown in Table 1. We specify the true number of topics for RECOVER-L2, RECOVER-KL and LDA while TOP estimates it.

The results have essentially the same pattern as those from the NIPs dataset. For the Dirichlet distribution with parameter 0.03, RECOVER-KL, RECOVER-L2 and TOP are comparable, whereas TOP outperforms the other two when the topics become more correlated. LDA has the worst performance, especially when  $n$  is relatively small. TOP and RECOVER-L2 run much faster than RECOVER-KL and LDA.

**Table 1.** Running time (seconds) of different algorithms on the NYT dataset

|             | TOP   | RECOVER-L2 | RECOVER-KL | LDA     |
|-------------|-------|------------|------------|---------|
| $n = 40000$ | 471.5 | 795.6      | 4681.9     | 35913.7 |
| $n = 50000$ | 517.2 | 841.5      | 4824.0     | 44754.1 |
| $n = 60000$ | 555.3 | 894.1      | 4945.3     | 53833.8 |
| $n = 70000$ | 579.2 | 957.2      | 5060.8     | 62548.8 |

**Real data comparison from the NYT dataset.** We applied TOP, RECOVER-L2, RECOVER-KL and LDA to the preprocessed NYT dataset. In order to ensure that all algorithms make use of a similar number of topics, TOP uses  $C_0 = 0.01$  and  $C_1 = 15.5$ , which gives an estimated  $\hat{K} = 101$ , and the other three algorithms use  $K = 101$  as input. Evaluation of algorithms on the real data is difficult since we do not know the ground truth. However, there exists some standard ways of evaluating the fitted model.

<sup>1</sup>The value of  $C_1$  is chosen such that the estimated number of topics is around 100

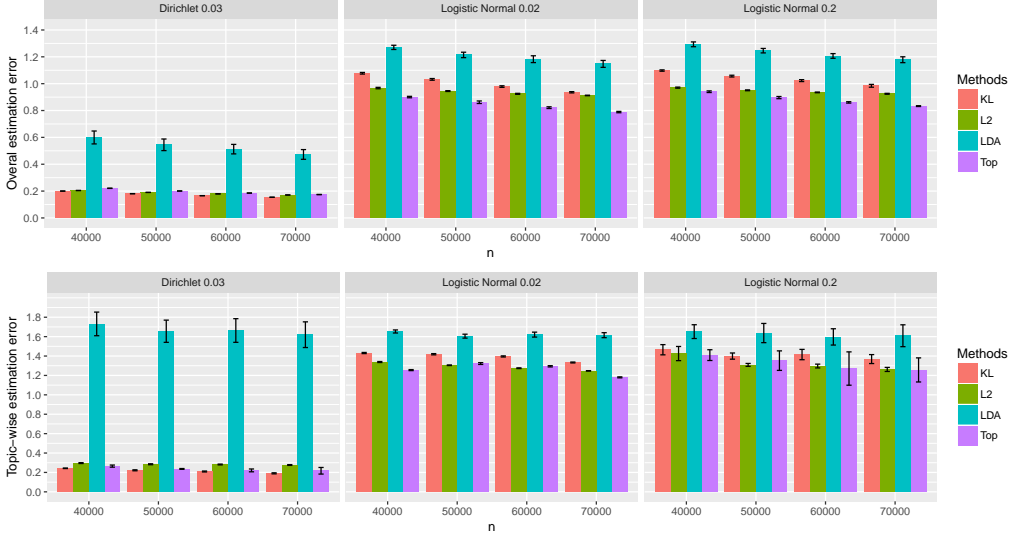

Figure 3: Plots of averaged *overall estimation error* and *topic-wise estimation error* of TOP, RECOVER-L2 (L2), RECOVER-KL (KL) and LDA from the NYT dataset. TOP estimates  $K$  while the other algorithms use the true  $K$  as input. The bars denote one standard deviation.

Since our main target is the word-topic matrix  $A$ , we consider two widely used metrics of evaluating the semantic quality of estimated topics <sup>2</sup> [1, 4, 5]:

- (1) *Topic coherence*. Coherence is a measure of the co-occurrence of the high-frequency words for each individual estimated topics. “This metric has been shown to correlate well with human judgments of topic quality. When the topics are perfectly recovered, all the high-probability words in a topic should co-occur frequently, otherwise, the model may be mixing unrelated concepts.” [1]. Given a set of words  $\mathcal{W}$ , coherence is calculated as

$$Coherence(\mathcal{W}) := \sum_{w_1, w_2 \in \mathcal{W}} \log \frac{D(w_1, w_2) + \varepsilon}{D(w_2)} \quad (82)$$

where  $D(w_1)$  denotes the number of documents that the word  $w_1$  occurs,  $D(w_1, w_2)$  denotes the number of documents that both word  $w_1$  and word  $w_2$  occur [4] and the parameter  $\varepsilon = 0.01$  is used to avoid taking the log of zero [5].

In the NYT dataset, for each algorithm, we use its estimated word-topic matrix  $\hat{A}$  and calculate  $Coherence(\mathcal{W}_k)$  for  $1 \leq k \leq \hat{K}$ , where  $\mathcal{W}_k$  is the set of 20 most frequent words in topic  $k$ . The averaged coherence metrics and its standard deviation

<sup>2</sup>We do not consider the metric of *held-out-probability* since it requires the estimation of both  $A$  and  $W$  while neither TOP nor RECOVER estimates  $W$ .

tion across topics of TOP, RECOVER and LDA are reported in Table 2.<sup>3</sup> TOP has the largest coherence suggesting a better topic recovery while RECOVER has the smallest coherence.

- (2) *Unique words*: Since coherence only measures the quality of each individual topic, we consider the metric, *unique words* [1], which reflects the redundancy between topics. For each topic and its  $T$  most probable words, we count how many of those  $T$  words do not appear in any  $T$  most probable words of the other topics. Some overlap across topics is expected due to semantic ambiguity, but lower numbers of unique words indicate less useful models. We consider  $T = 100$  and the averaged unique words and the standard deviation across topics are reported in Table 2. TOP and LDA have more unique words than RECOVER. In fact, the unique words from RECOVER are only the anchor words and the other most probable words of different topics are all overlapped, indicating the redundancy between the estimated topics.

**Table 2.** Coherence and unique words of TOP, RECOVER and LDA on the NYT dataset. The numbers in the parentheses are the standard deviations across topics.

| Metric              | TOP          | RECOVER     | LDA          |
|---------------------|--------------|-------------|--------------|
| <i>Coherence</i>    | -328.8(51.3) | -464.1(3.8) | -340.3(44.8) |
| <i>Unique words</i> | 6.7(4.4)     | 1.0(0.0)    | 6.3(3.1)     |

## References

- [1] ARORA, S., GE, R., HALPERN, Y., MIMNO, D. M., MOITRA, A., SONTAG, D., WU, Y. and ZHU, M. (2013). A Practical Algorithm for Topic Modeling with Provable Guarantees. In *ICML (2)* 280–288.
- [2] BING, X., BUNEA, F., YANG, N. and WEGKAMP, M. (2017). Sparse Latent Factor Models with Pure Variables for Overlapping Clustering. *arXiv: 1704.06977*.
- [3] KE, T. Z. and WANG, M. (2017). A new SVD approach to optimal topic estimation. *arXiv:1704.07016*.
- [4] MIMNO, D., WALLACH, H. M., TALLEY, E., LEENDERS, M. and MCCALLUM, A. (2011). Optimizing Semantic Coherence in Topic Models. In *Proceedings of the Conference on Empirical Methods in Natural Language Processing. EMNLP '11* 262–272. Association for Computational Linguistics, Stroudsburg, PA, USA.
- [5] STEVENS, K., KEGELMEYER, P., ANDRZEJEWSKI, D. and BUTTLER, D. (2012). Exploring Topic Coherence over Many Models and Many Topics. In *Proceedings of the 2012 Joint Conference on Empirical Methods in Natural Language Processing and Computational Natural Language Learning* 952–961. Association for Computational Linguistics, Jeju Island, Korea.
- [6] TSYBAKOV, A. B. (2009). *Introduction to Nonparametric Estimation*. Springer, New York.

<sup>3</sup>We only report one of RECOVER-L2 and RECOVER-KL since they have the same results.
